# Supplementary material for: Scarce Data, Noisy Inferences, and Overfitting: The Hidden Flaws in Ecological Dynamics Modelling
Source: arXiv:2510.03718 ancillary file (2025-10-04)
Supplement: Supplementary file 1 [file SI.pdf]

Journal of the Royal Society Interface



# Supplementary Information: Scarce Data, Noisy Inferences, and Overfitting: The Hidden Flaws in Ecological Dynamics Modelling

Mario Castro[1,2], Rafael Vida[1,2,4], Javier Galeano[2,4], José A. Cuesta[2,3,5]

[1]Institute for Research in Technology (IIT), Universidad Pontificia Comillas, Madrid, Spain
[2]Grupo Interdisciplinar de Sistemas Complejos (GISC), Madrid, Spain
[3]Universidad Carlos III de Madrid, Departamento de Matemáticas, Leganés, Spain
[4]Complex System Group, Universidad Politécnica de Madrid, Madrid, Spain
[5]Instituto de Biocomputación y Física de Sistemas Complejos, Universidad de Zaragoza, Zaragoza, Spain

royalsocietypublishing.org/journal/rsif J R Soc Interface 0000000

# S1. Parameters used in the simulation

In Table S1, we collect the parameters used to simulate Eq. (S1):

$$\frac{dx_i}{dt} = x_i\left(r_i + \sum_{j=1}^{N} \beta_{ij} x_j\right), \quad i = 1 \dots N, \tag{S1}$$

and the main figure corresponding to those parameters. In the case of the simulations used to apply Bayesian inference, the code is freely available at https://zenodo.org/records/16747311, so we indicate the random seed used in the simulations (for reproducibility). Recall that

- $x_i$ represents the population size of species $i$,
- $r_i$ is the intrinsic growth rate of species $i$,
- $\beta_{ij}$ denotes the interaction coefficient between species $i$ and $j$.

**Table S1.** Parameters used in this work. The first column points to the main figure related to those parameters. The seed used in the simulation code is shown in the case of those used to make Bayesian inference. The numbers have been rounded to the second significant figure for compactness.

| Main figure | $x_i(0)$ | $r_i$ | $\beta_{ij}$ | Reference |
|---|---|---|---|---|
| 3 (main text) | $\begin{bmatrix}0.22\\0.063\\0.0014\end{bmatrix}$ | $\begin{bmatrix}1.1\\3.9\\0.78\end{bmatrix}$ | $\begin{bmatrix}-1.8 & 1.2 & -1.7\\-1.5 & -2.6 & 0.35\\-0.12 & 1.3 & -2.7\end{bmatrix}$ | This work (seed 434) |
| 5 (main text) | $\begin{bmatrix}10\\10\\10\\10\end{bmatrix}$ | $\begin{bmatrix}-0.16\\-0.63\\-0.82\\1.9\end{bmatrix}$ | $\begin{bmatrix}0.29 & -1.8 & -0.21 & 1.5\\0.92 & -2.0 & -0.22 & 0.48\\1.8 & 0.65 & -1.5 & -1.3\\1.4 & -1.3 & -0.32 & -1.4\end{bmatrix}$ | This work |
| S19 | $\begin{bmatrix}0.017\\0.037\\0.16\\0.058\end{bmatrix}$ | $\begin{bmatrix}0.47\\1.8\\2.6\\0.64\end{bmatrix}$ | $\begin{bmatrix}-0.14 & 0.38 & 0.22 & -0.43\\-1.4 & -1.2 & 0.023 & -1.1\\2.2 & 1.7 & -2.8 & -0.044\\-0.76 & 2.0 & 0.24 & -0.78\end{bmatrix}$ | This work (seed 64977) |
| S20 | $\begin{bmatrix}0.049\\0.025\\0.04\\0.011\\0.11\end{bmatrix}$ | $\begin{bmatrix}2.7\\6.1\\0.60\\2.2\\0.70\end{bmatrix}$ | $\begin{bmatrix}-8.2 & 0.74 & 1.7 & 0.09 & -0.37\\0.15 & -1.9 & 0.37 & 0.56 & -0.42\\-0.49 & 0.31 & -4.3 & 0.33 & 0.15\\-1.1 & -0.45 & 1.4 & -4.4 & 2.7\\-0.95 & 0.67 & -0.52 & -0.80 & -0.95\end{bmatrix}$ | This work (seed 74435) |
| S24 | $\begin{bmatrix}11\\14\\1\end{bmatrix}$ | $\begin{bmatrix}0.25\\-0.50\\-0.50\end{bmatrix}$ | $\begin{bmatrix}-0.0010 & -0.040 & -0.040\\0.040 & -0.0020 & -0.020\\0.020 & 0.040 & -0.0030\end{bmatrix}$ | This work |
| S25 | $\begin{bmatrix}10\\14\\4\end{bmatrix}$ | $\begin{bmatrix}6\\4\\2\end{bmatrix}$ | $\begin{bmatrix}-0.05 & 0.15 & -0.20\\-0.01 & -0.027 & 0.050\\0.10 & -0.10 & -0.015\end{bmatrix}$ | [1] |
| S26 | $\begin{bmatrix}0.04\\0.04\\0.12\\0.04\\0.03\\0.07\end{bmatrix}$ | $\begin{bmatrix}2.4\\0.005\\0.4\\4.3\\0.5\\1.7\end{bmatrix}$ | $\begin{bmatrix}-0.48 & -0.09 & 1.6 & -1.5 & -1.8 & 1.7\\1.3 & -0.1 & -1.1 & 1.2 & -0.72 & -1.6\\-0.5 & 1.1 & -1 & 2.9 & -1.3 & 0.67\\0.42 & 0.13 & -0.9 & -0.42 & -1.1 & 1.1\\0.18 & 1.6 & 1.7 & -0.09 & -3.5 & 0.005\\-0.11 & 0.55 & -1.4 & 1.9 & -0.65 & -3.5\end{bmatrix}$ | This work (seed 72088) |

## S2. Bayesian inference



royalsocietypublishing.org/journal/rsif J R Soc Interface 000000

We consider an $N$-species generalised Lotka-Volterra model where the population dynamics are governed by the system of differential equations in Eqs. (S1).

Here, we introduce a novel approach to model this using an approximate numerical solution combined with a log-normally distributed noise (as discussed in the main text). Thus, we proceed in two steps: (a) we apply a classical fourth-order Runge-Kutta (RK4) integrator to generate prospect abundances for each species, and (b) we generate the abundances at the next time step through a Bayesian hierarchical model. We detail these two steps in what follows.

### (a) Fourth-order Runge-Kutta integrator

Given the abundances $x_{n-1,i}$ at time step $n-1$, we compute

$$k_{1,i} = x_{n-1,i}\left(r_i + \sum_{j=1}^{N} \beta_{ij} x_{n-1,j}\right), \tag{S1}$$

$$k_{2,i} = \left(x_{n-1,i} + \frac{dt}{2}k_{1,i}\right)\left(r_i + \sum_{j=1}^{N} \beta_{ij} x^{(1)}_{n-1,i}\right), \tag{S2}$$

$$k_{3,i} = \left(x_{n-1,i} + \frac{dt}{2}k_{2,i}\right)\left(r_i + \sum_{j=1}^{N} \beta_{ij} x^{(2)}_{n-1,i}\right), \tag{S3}$$

$$k_{4,i} = \left(x_{n-1,i} + dt k_{3,i}\right)\left(r_i + \sum_{j=1}^{N} \beta_{ij} x^{(3)}_{n-1,i}\right). \tag{S4}$$

where

$$x^{(r)}_{n-1,j} = x_{n-1,j} + \frac{dt}{2}k_{r,j}, \quad r = 1, 2, 3, \tag{S5}$$

and produce

$$x^{*}_{n,i} = x_{n-1,i} + \frac{dt}{6}(k_{1,i} + 2k_{2,i} + 2k_{3,i} + k_{4,i}). \tag{S6}$$

### (b) Bayesian hierarchical model

The parameters of the model follow prior distributions:

$$\sigma_i \sim \text{Exponential}(1), \tag{S7}$$

$$r_i \sim \text{Exponential}(0.1), \tag{S8}$$

$$\beta_{ij} \sim \mathcal{N}(0, 2). \tag{S9}$$

Given the population values $x_{n,i}$ obtained via RK4, the likelihood function assumes:

$$x_{n,i} \sim \text{Lognormal}(\log x^{*}_{n,i}, \sigma_i), \tag{S10}$$

with the $x^{*}_{n,i}$ obtained in (S6)

# S3. Marginal posterior distributions

## (a) 3 species

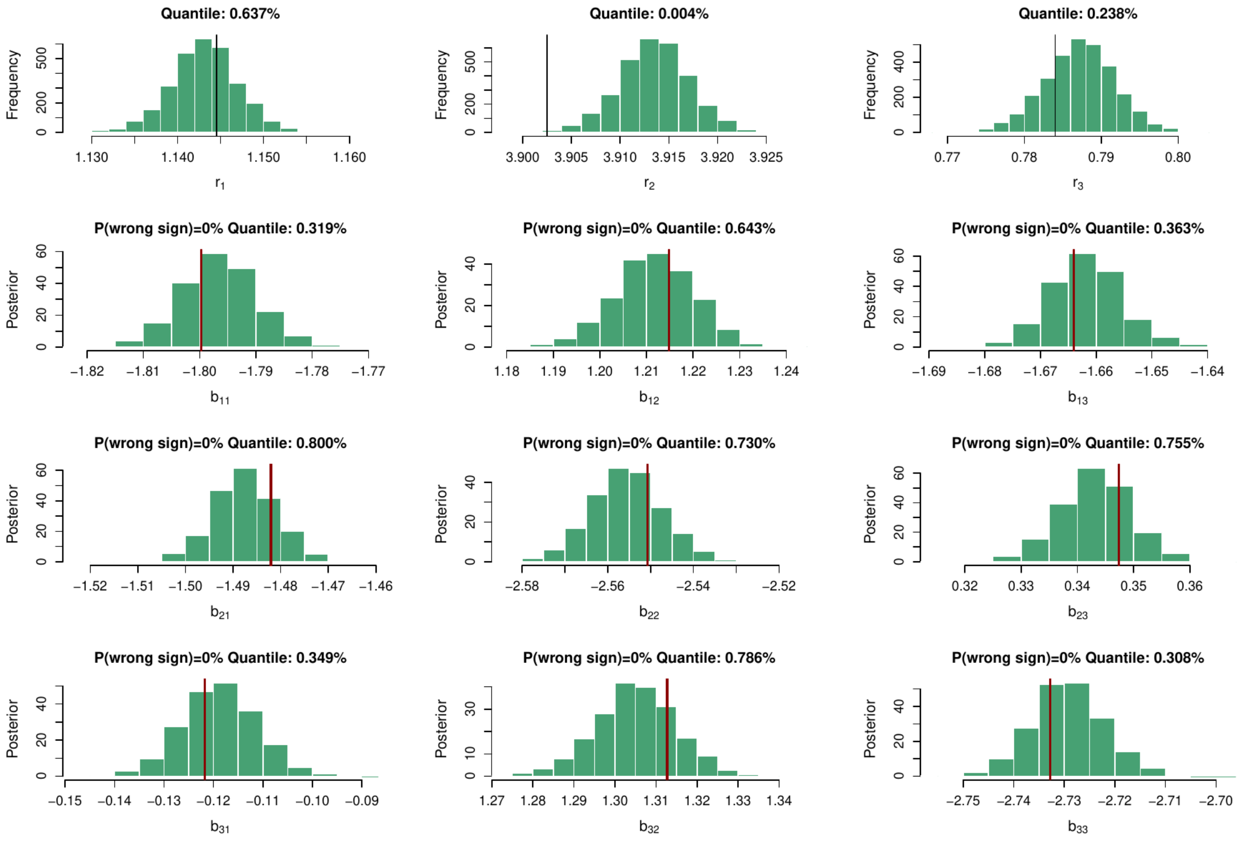


**Figure S1.** Marginals of the posterior distributions for the parameters of the gLV adding log-normal noise with standard deviation 0.001. The vertical red line is the original parameter value used in the simulation.

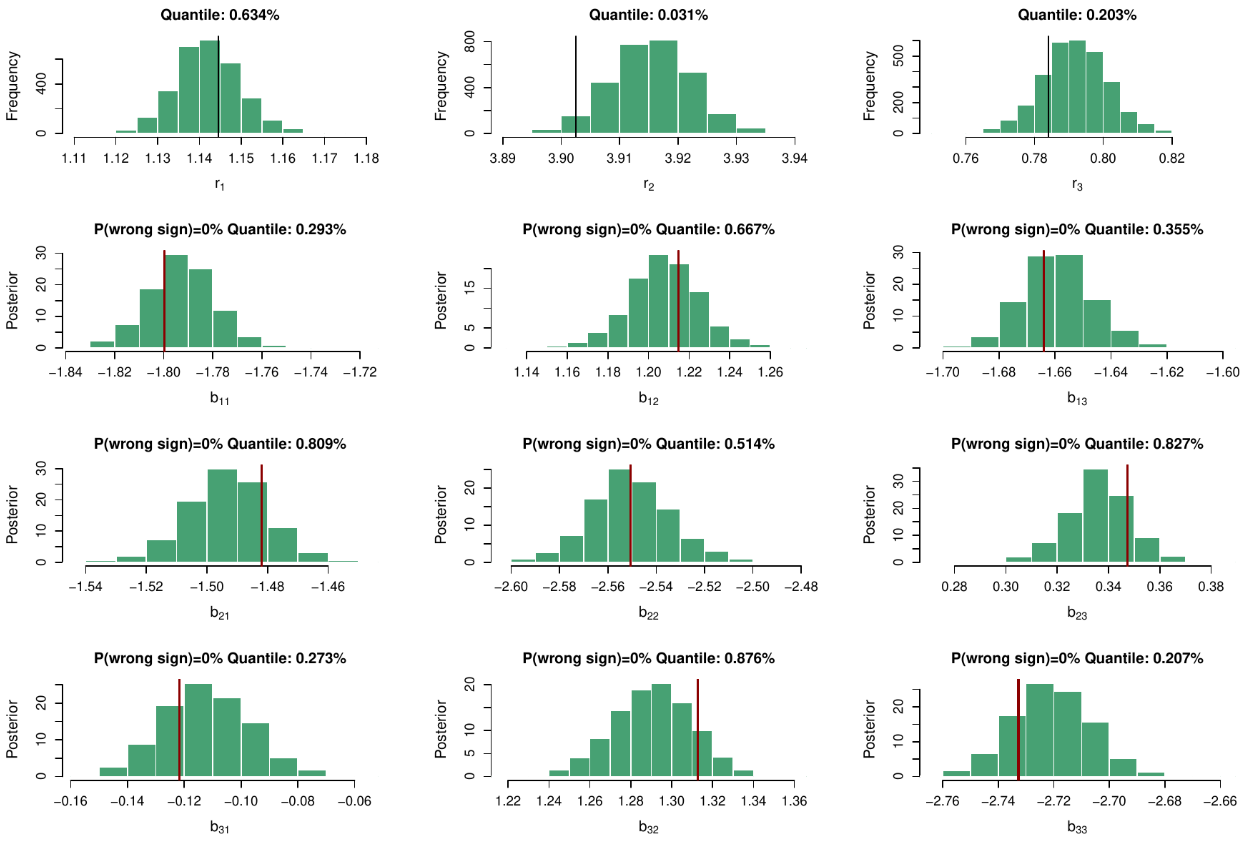


**Figure S2.** Marginals of the posterior distributions for the parameters of the gLV adding log-normal noise with standard deviation 0.002. The vertical red line is the original parameter value used in the simulation. In purple, we show those ranges of parameters that have a change of sign.

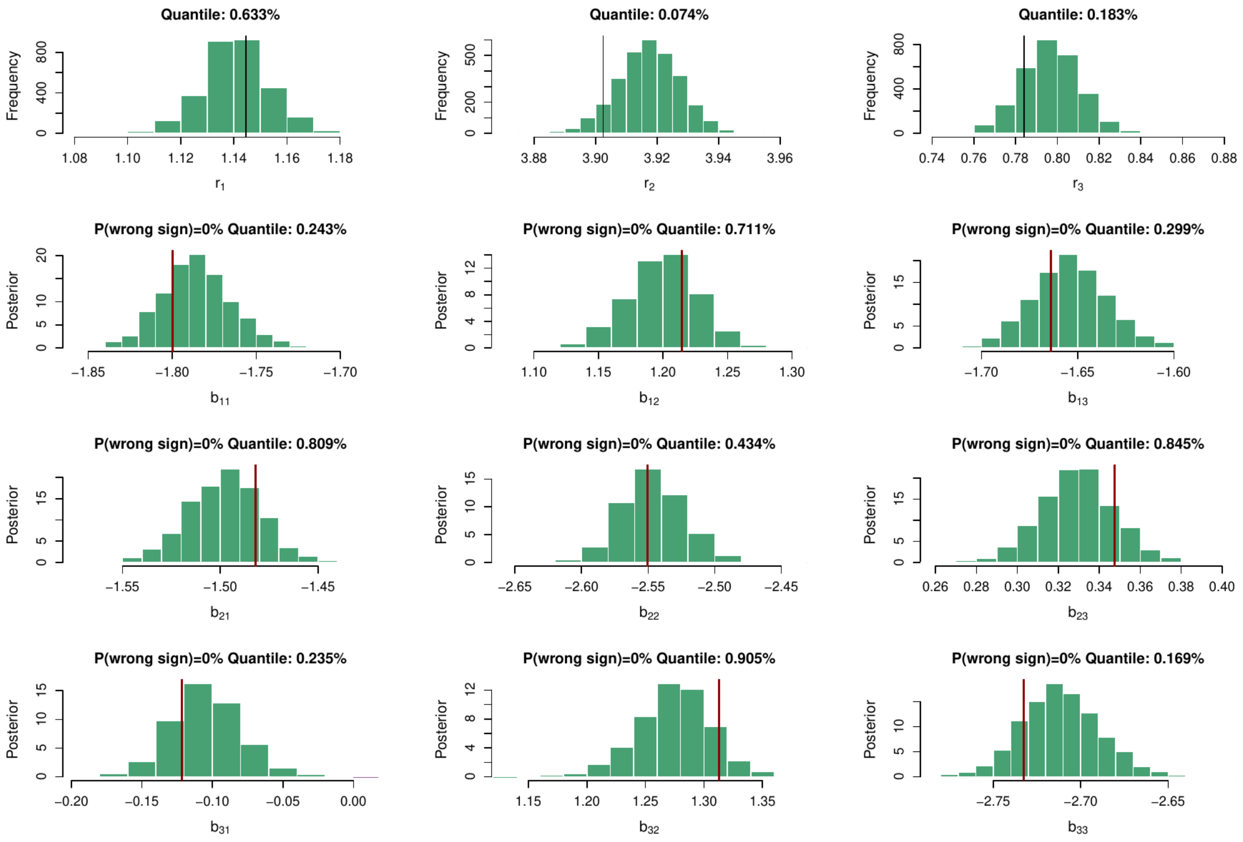


**Figure S3.** Marginals of the posterior distributions for the parameters of the gLV adding log-normal noise with standard deviation 0.003. The vertical red line is the original parameter value used in the simulation. In purple, we show those ranges of parameters that have a change of sign.

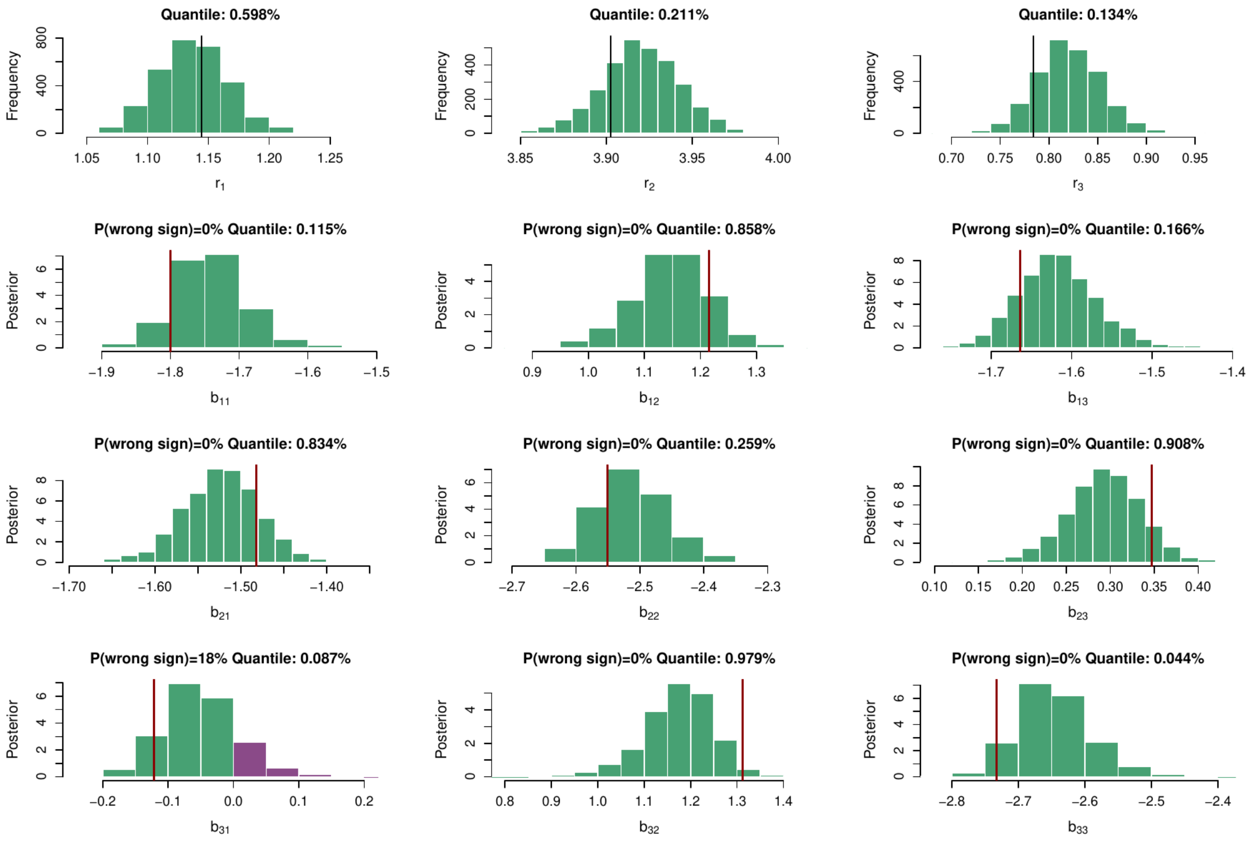


**Figure S4.** Marginals of the posterior distributions for the parameters of the gLV adding log-normal noise with standard deviation 0.007. The vertical red line is the original parameter value used in the simulation. In purple, we show those ranges of parameters that have a change of sign.

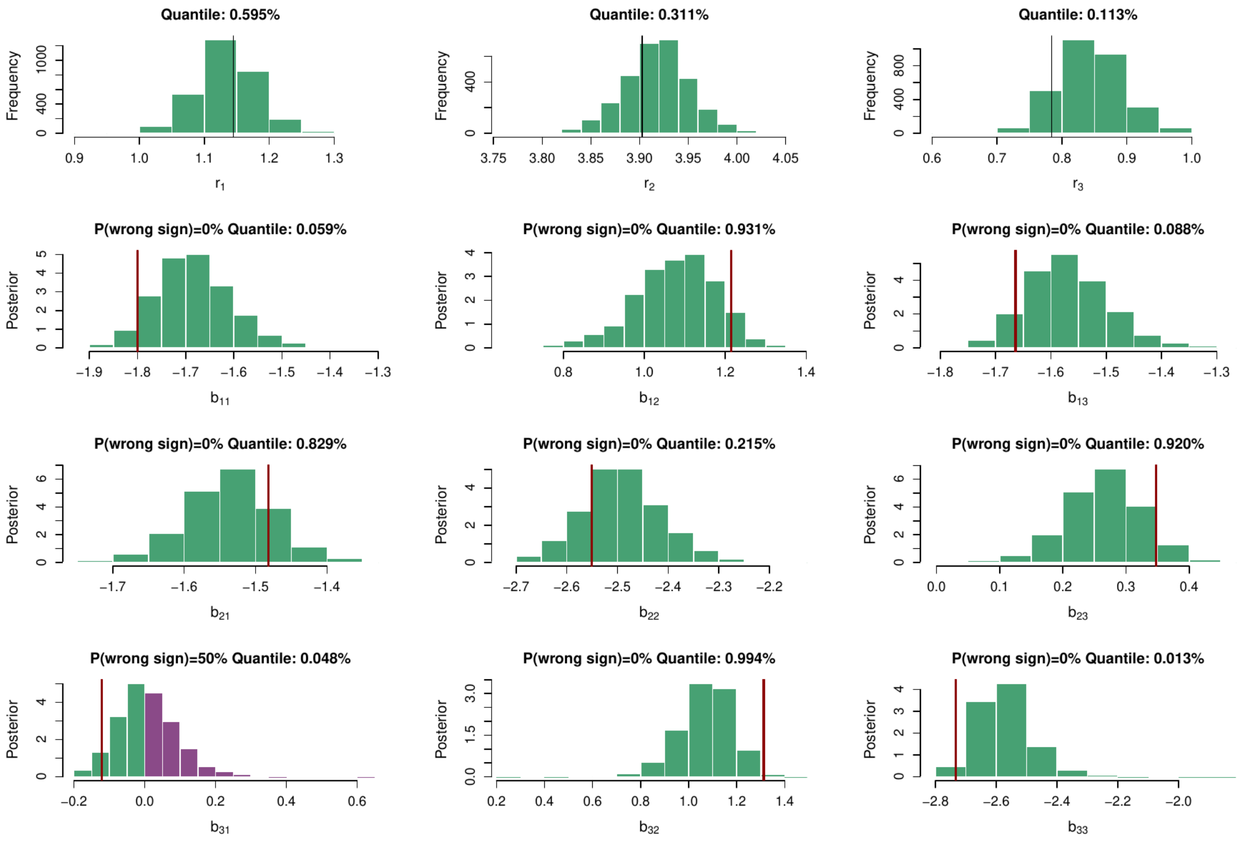


**Figure S5.** Marginals of the posterior distributions for the parameters of the gLV adding log-normal noise with standard deviation 0.01. The vertical red line is the original parameter value used in the simulation. In purple, we show those ranges of parameters that have a change of sign.

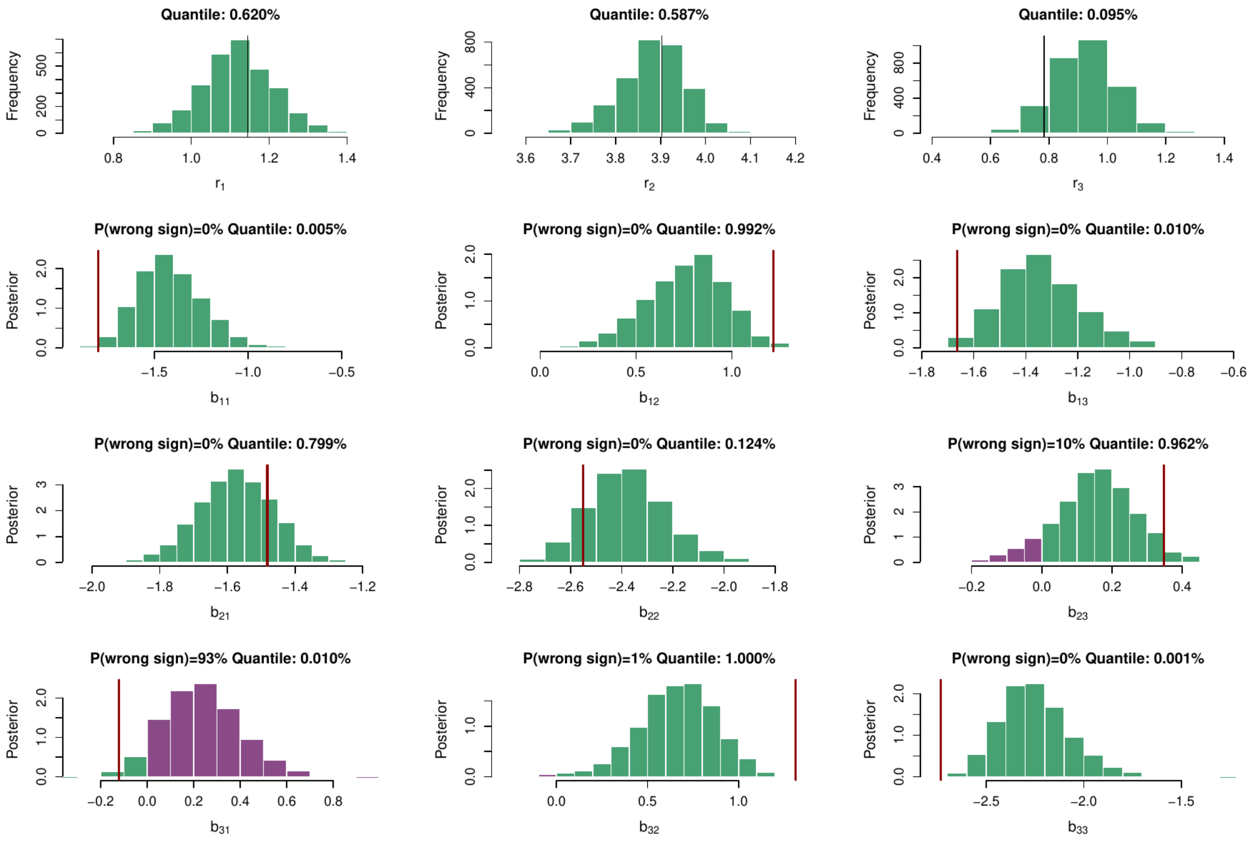


**Figure S6.** Marginals of the posterior distributions for the parameters of the gLV adding log-normal noise with standard deviation 0.02. The vertical red line is the original parameter value used in the simulation. In purple, we show those ranges of parameters that have a change of sign.

## (b) 4 species

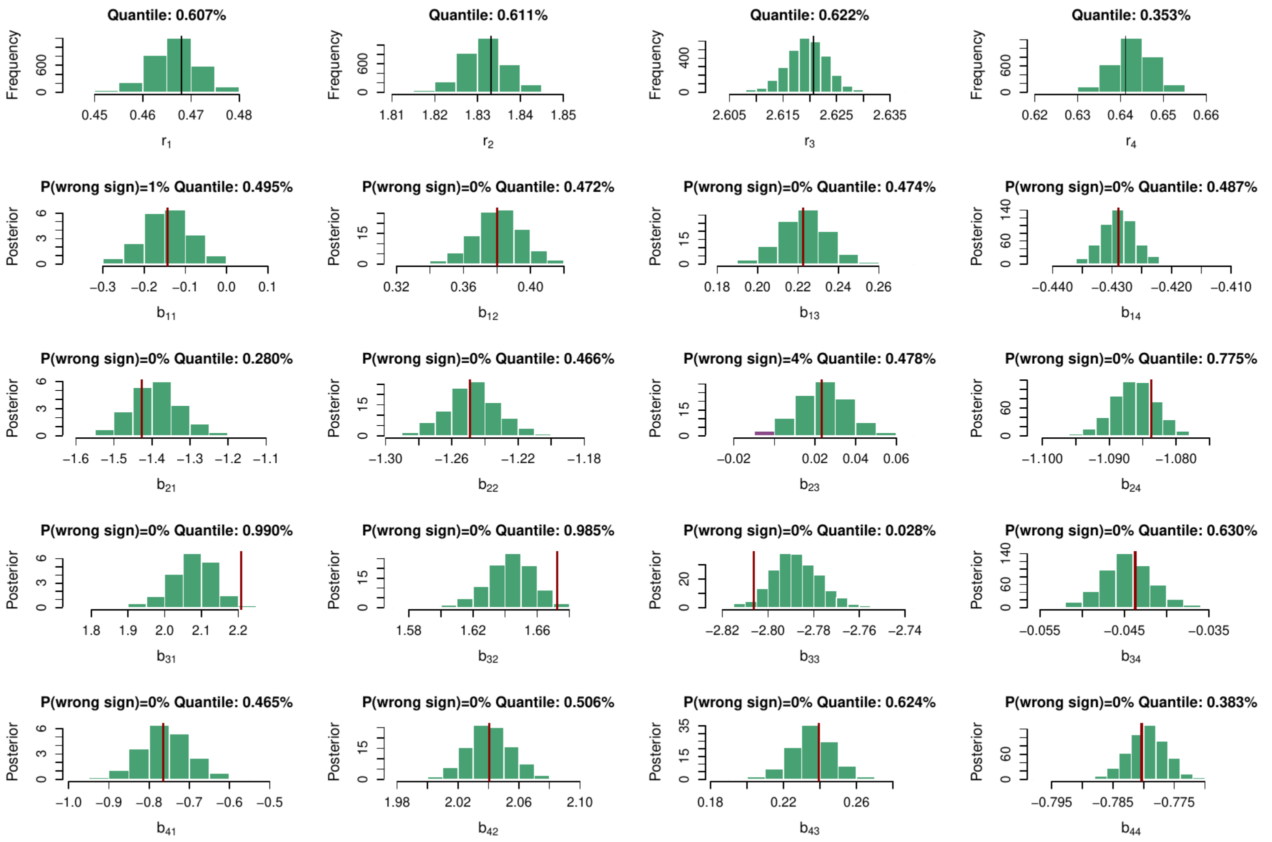


**Figure S7.** Marginals of the posterior distributions for the parameters of the gLV adding log-normal noise with standard deviation 0.001. The vertical red line is the original parameter value used in the simulation. In purple, we show those ranges of parameters that have a change of sign.

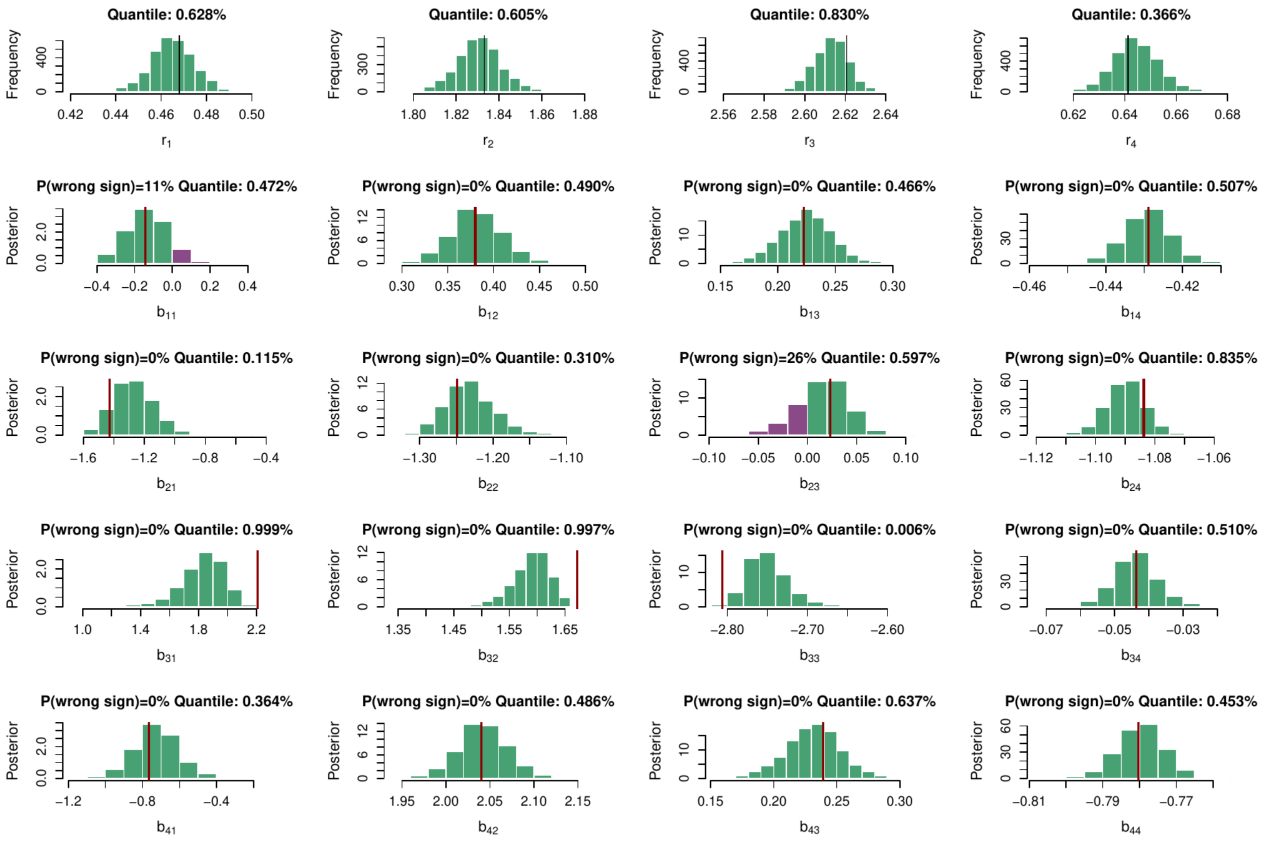


**Figure S8.** Marginals of the posterior distributions for the parameters of the gLV adding log-normal noise with standard deviation 0.002. The vertical red line is the original parameter value used in the simulation. In purple, we show those ranges of parameters that have a change of sign.

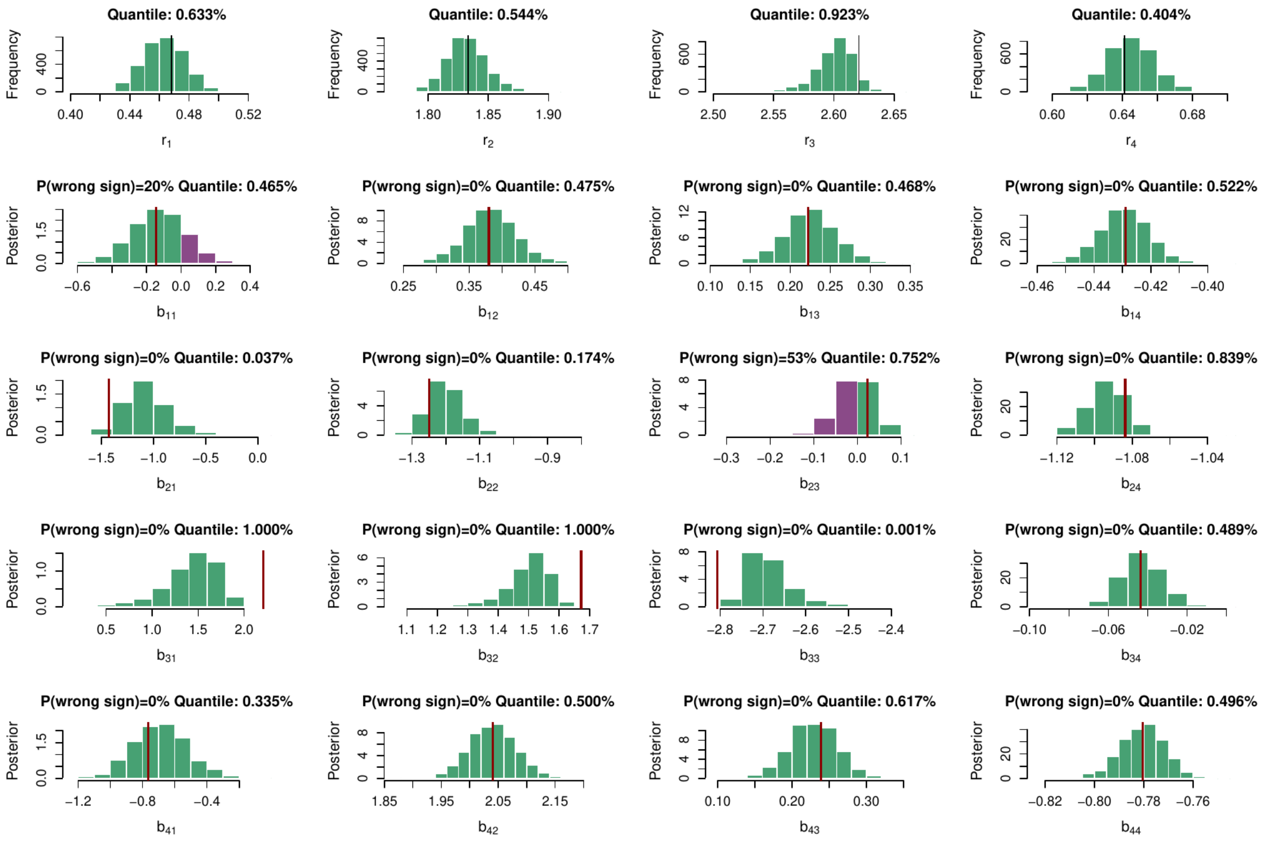


**Figure S9.** Marginals of the posterior distributions for the parameters of the gLV adding log-normal noise with standard deviation 0.003. The vertical red line is the original parameter value used in the simulation. In purple, we show those ranges of parameters that have a change of sign.

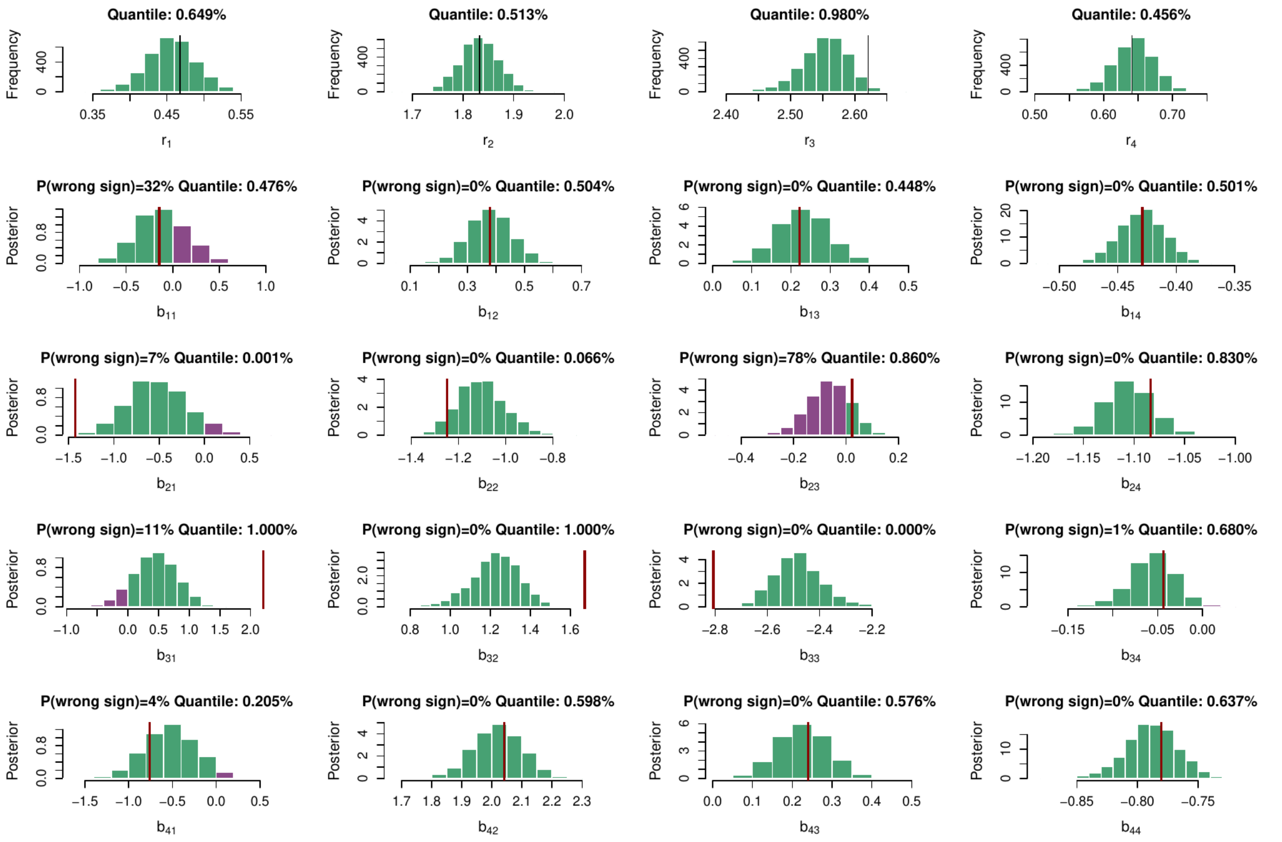


**Figure S10.** Marginals of the posterior distributions for the parameters of the gLV adding log-normal noise with standard deviation 0.007. The vertical red line is the original parameter value used in the simulation. In purple, we show those ranges of parameters that have a change of sign.

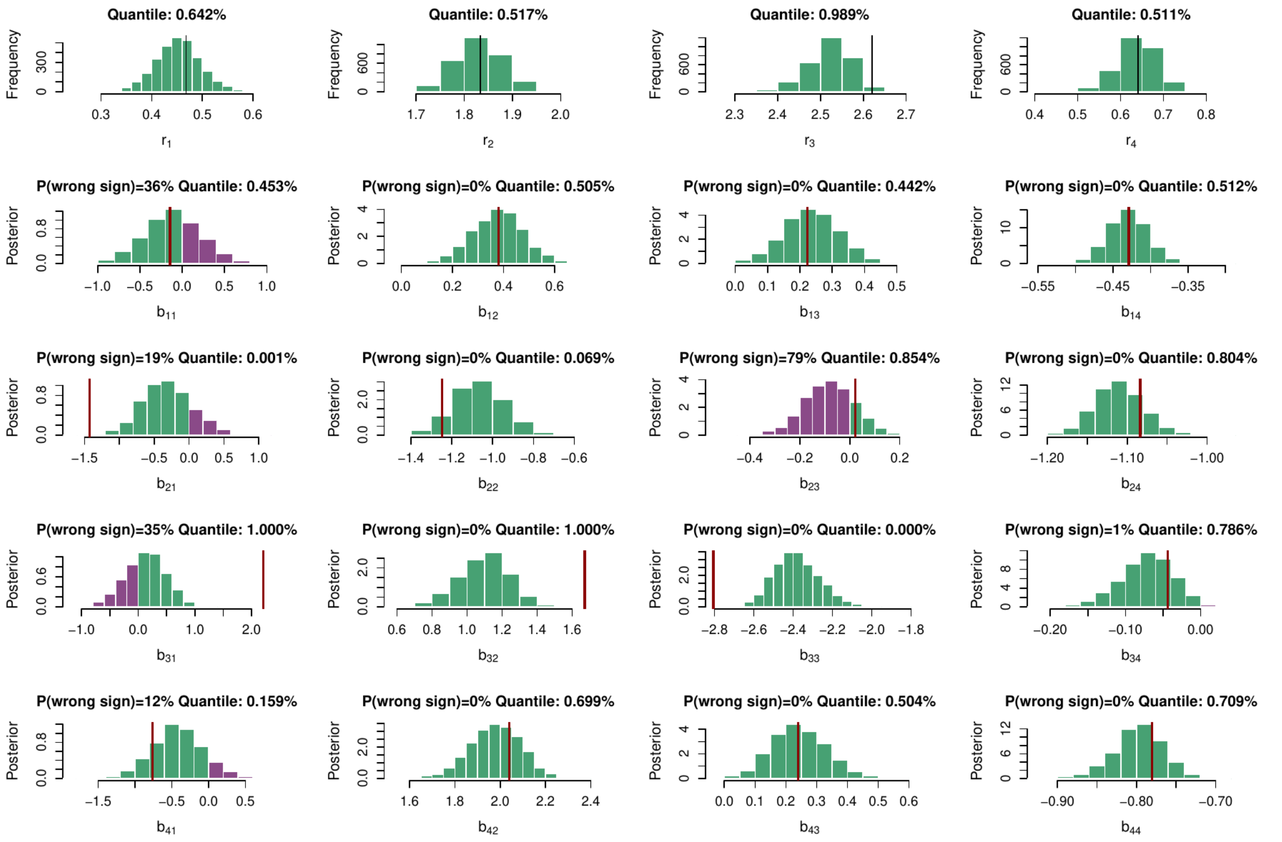


**Figure S11.** Marginals of the posterior distributions for the parameters of the gLV adding log-normal noise with standard deviation 0.01. The vertical red line is the original parameter value used in the simulation. In purple, we show those ranges of parameters that have a change of sign.

royalsocietypublishing.org/journal/rsif J R Soc Interface 0000000

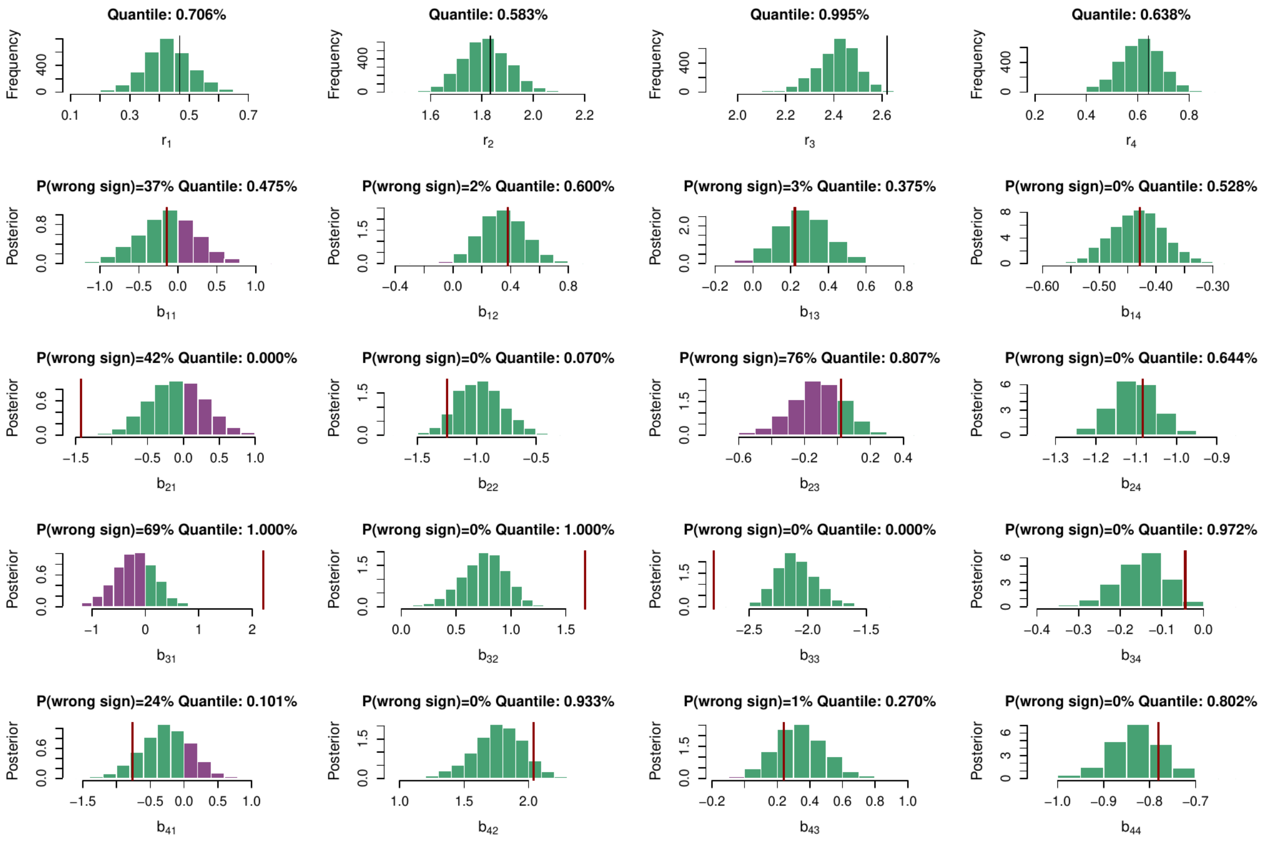


**Figure S12.** Marginals of the posterior distributions for the parameters of the gLV adding log-normal noise with standard deviation 0.02. The vertical red line is the original parameter value used in the simulation. In purple, we show those ranges of parameters that have a change of sign.

## (c) 5 species





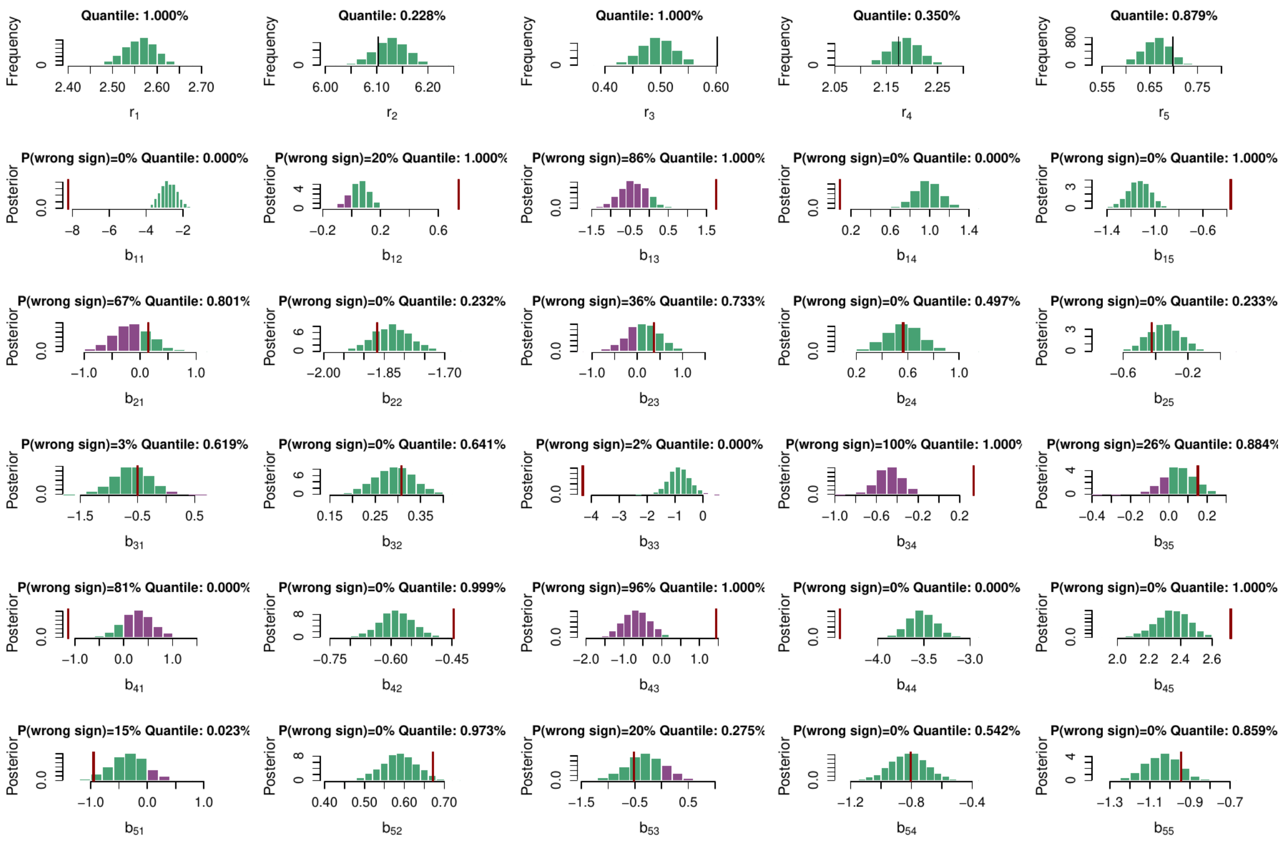

**Figure S13.** Marginals of the posterior distributions for the parameters of the gLV adding log-normal noise with standard deviation 0.001. The vertical red line is the original parameter value used in the simulation. In purple, we show those ranges of parameters that have a change of sign.

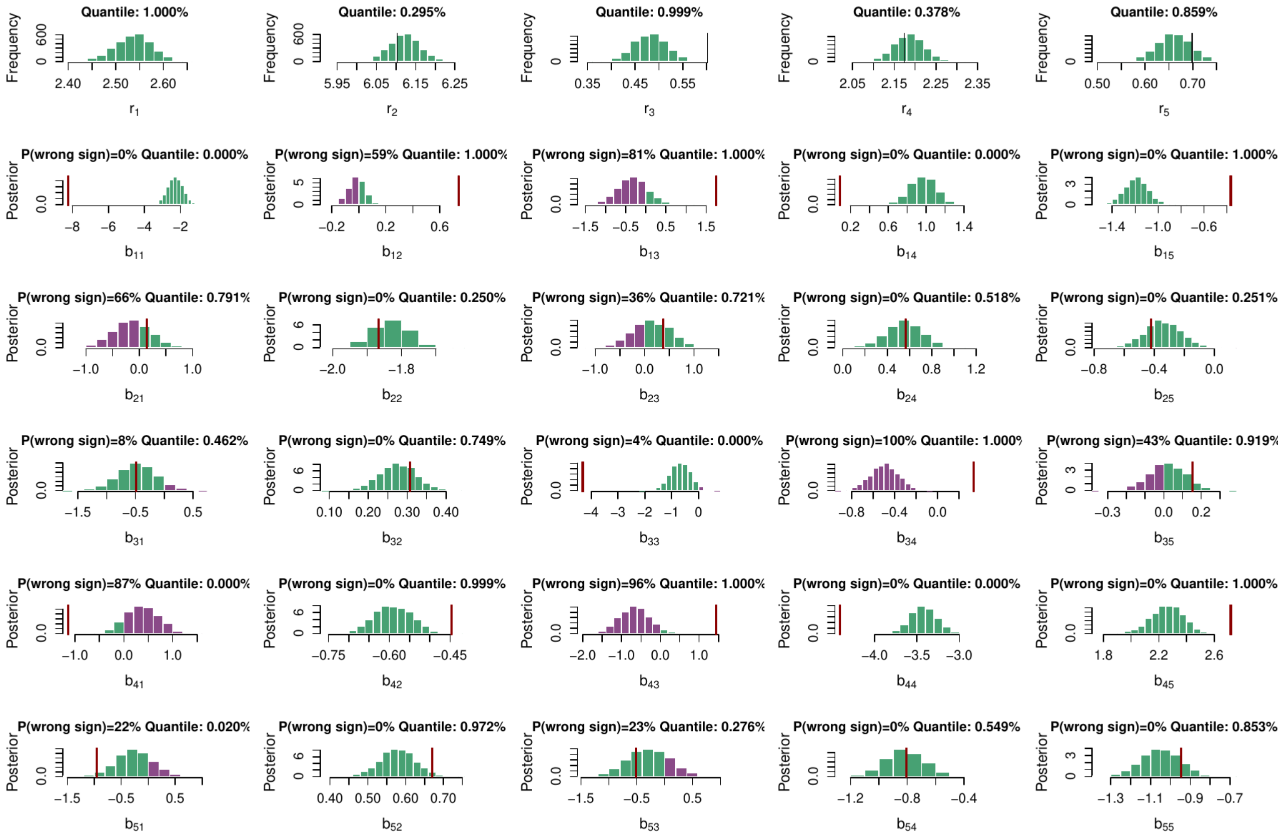


**Figure S14.** Marginals of the posterior distributions for the parameters of the gLV adding log-normal noise with standard deviation 0.002. The vertical red line is the original parameter value used in the simulation. In purple, we show those ranges of parameters that have a change of sign.

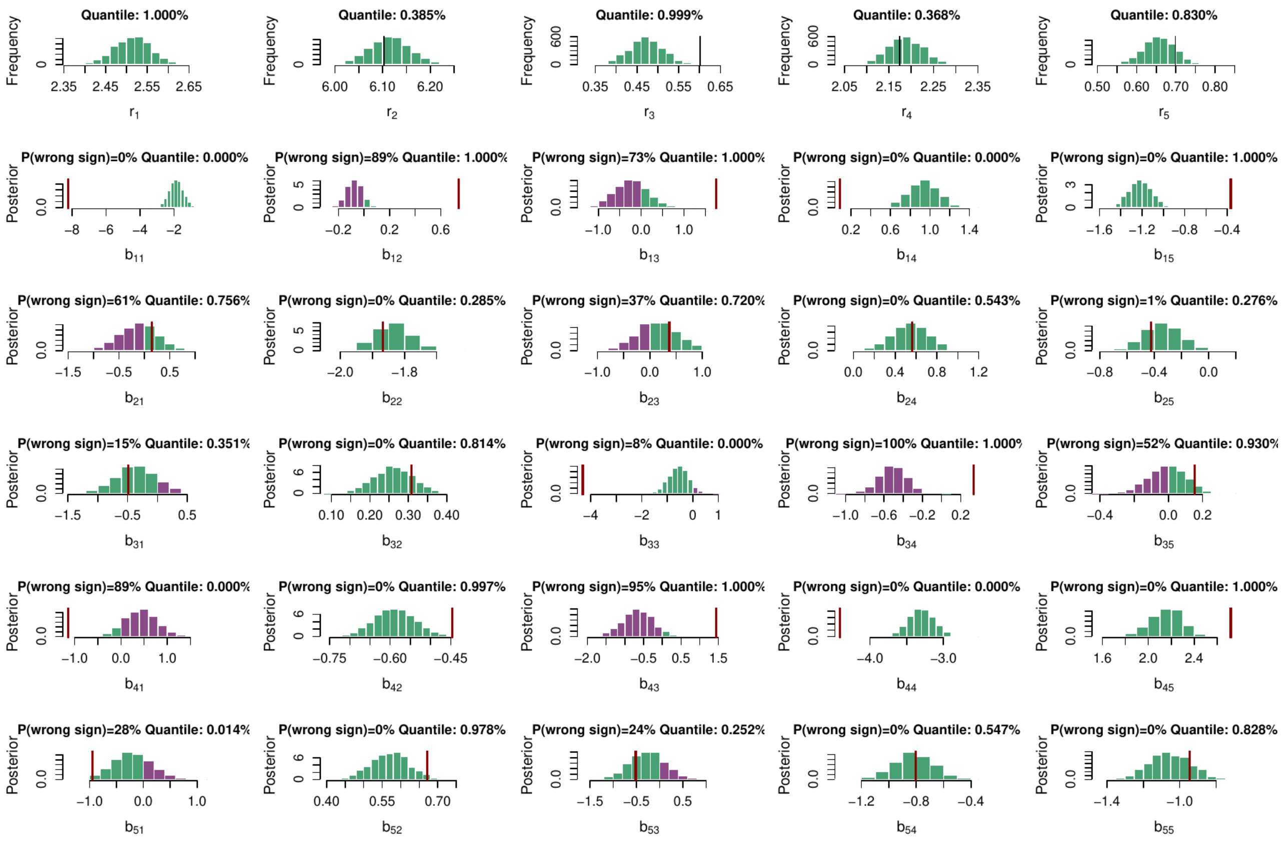

**Figure S15.** Marginals of the posterior distributions for the parameters of the gLV adding log-normal noise with standard deviation 0.003. The vertical red line is the original parameter value used in the simulation. In purple, we show those ranges of parameters that have a change of sign.

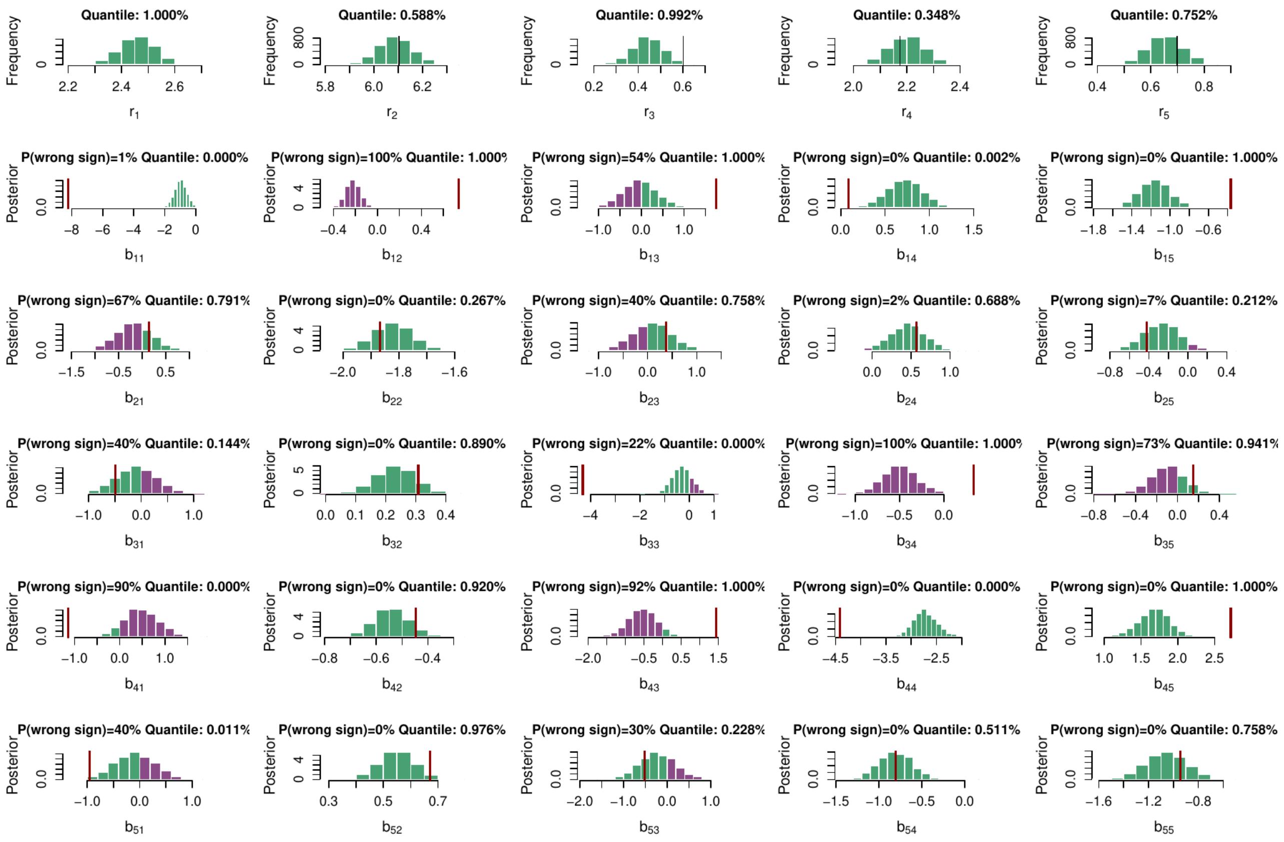


**Figure S16.** Marginals of the posterior distributions for the parameters of the gLV adding log-normal noise with standard deviation 0.007. The vertical red line is the original parameter value used in the simulation. In purple, we show those ranges of parameters that have a change of sign.

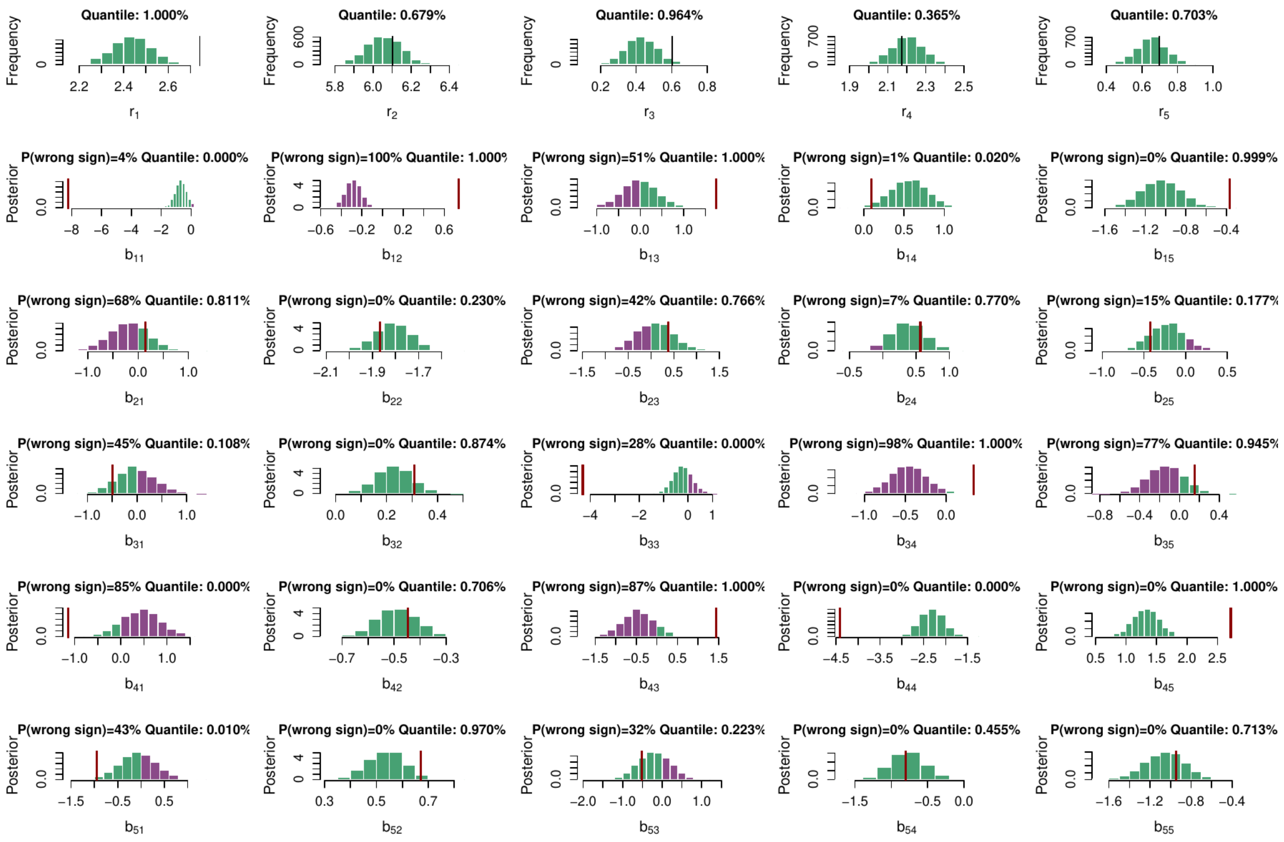


**Figure S17.** Marginals of the posterior distributions for the parameters of the gLV adding log-normal noise with standard deviation 0.01. The vertical red line is the original parameter value used in the simulation. In purple, we show those ranges of parameters that have a change of sign.

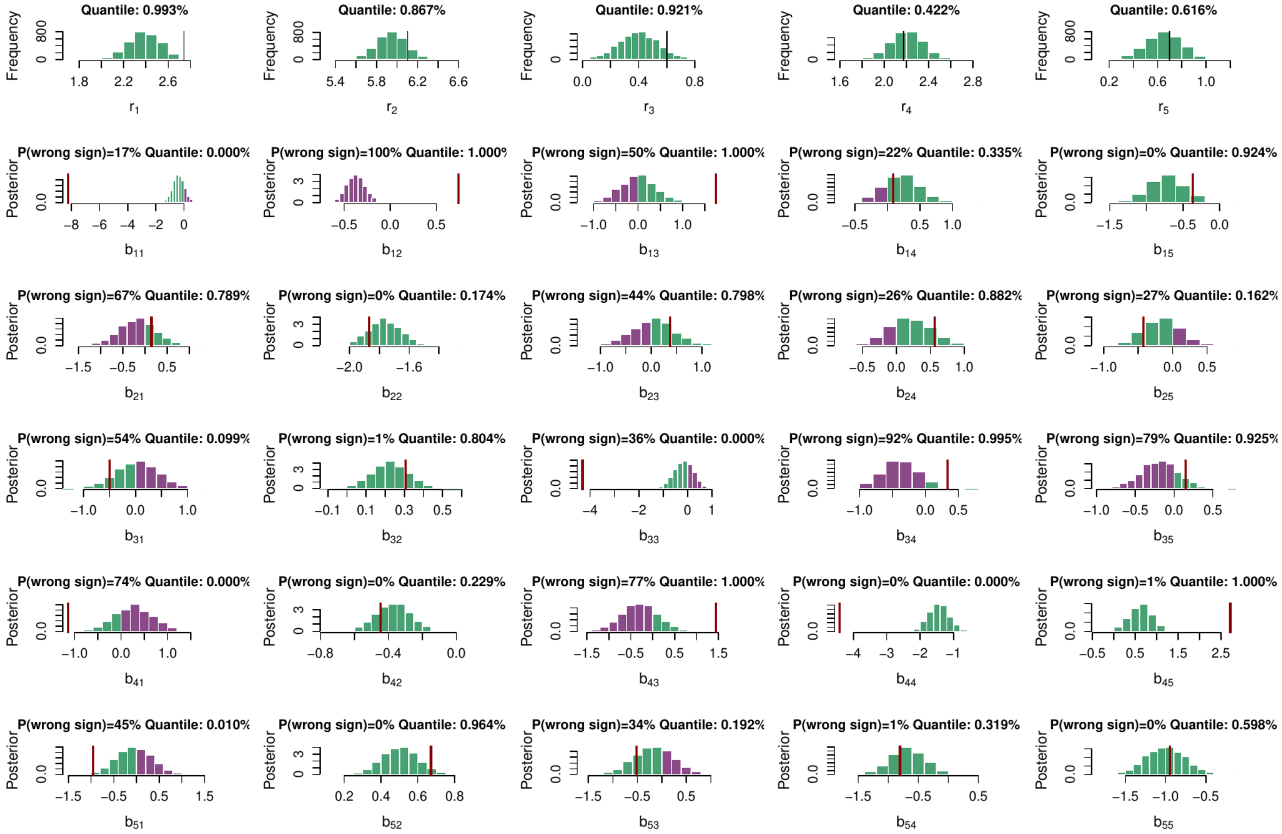

**Figure S18.** Marginals of the posterior distributions for the parameters of the gLV adding log-normal noise with standard deviation 0.02. The vertical red line is the original parameter value used in the simulation. In purple, we show those ranges of parameters that have a change of sign.

# S4. Posterior predictive checks

## (a) 4 species

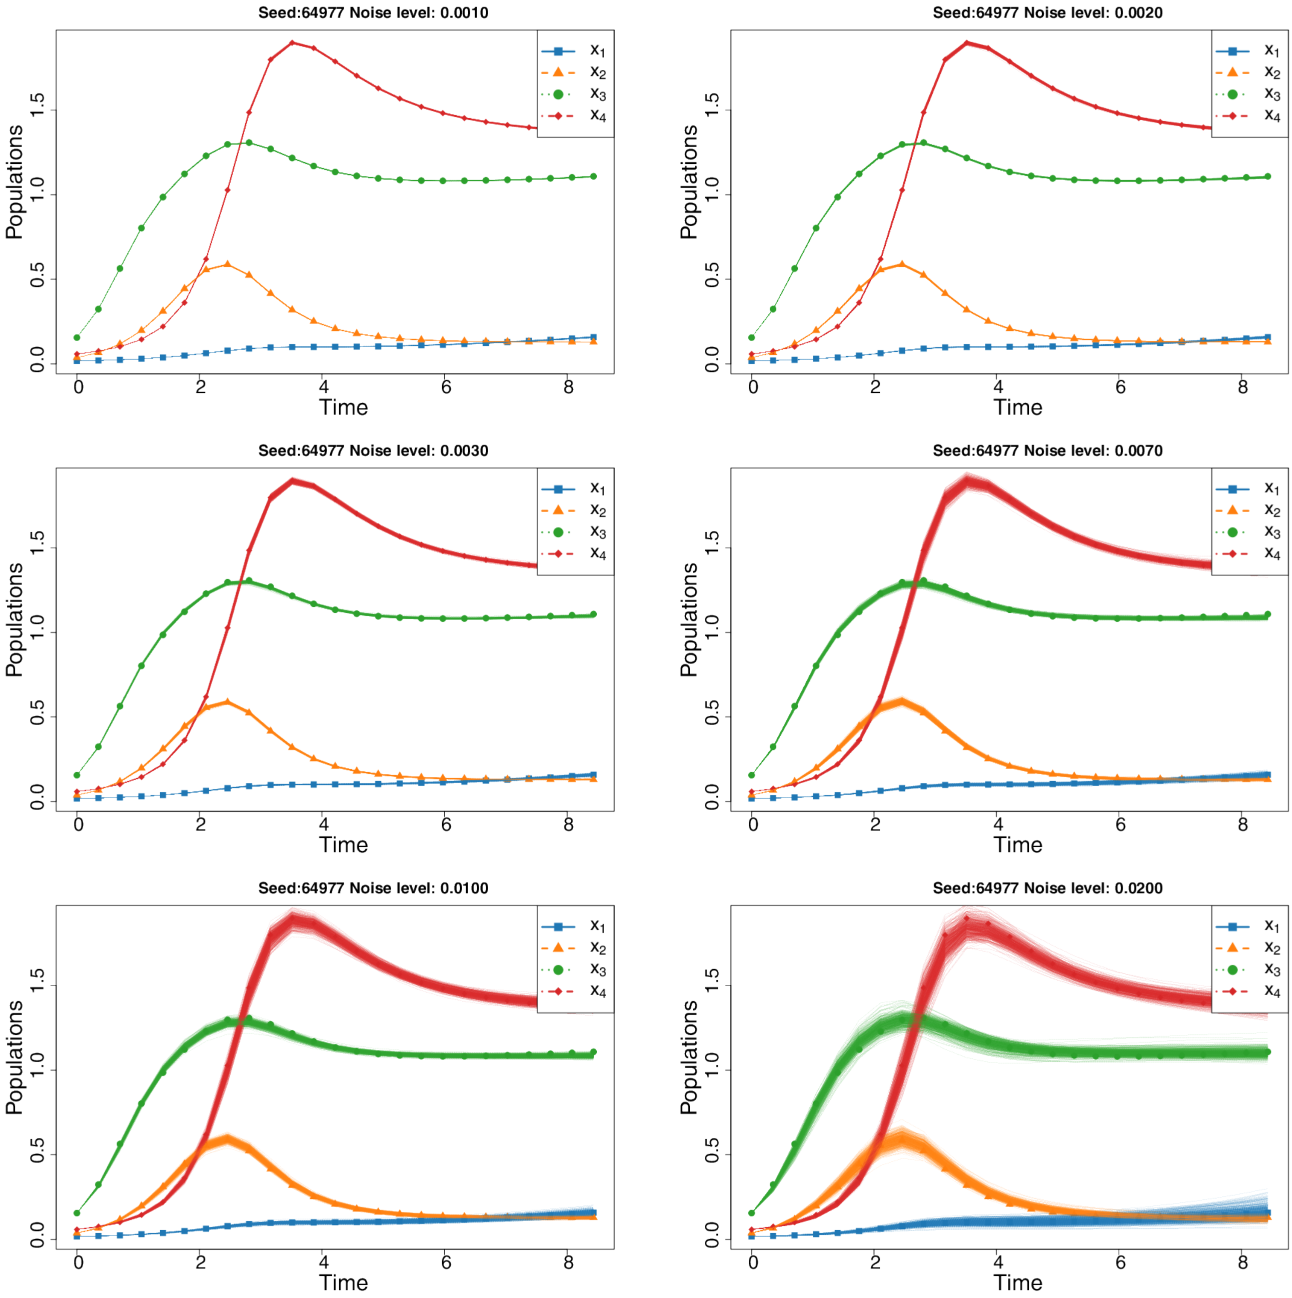


**Figure S19.** Posterior predictive trajectories simulated by sampling the posterior distributions (summarized in Sec. S3) for 6 different log-normally noise levels (title of each panel) added to the deterministic curves. The posterior predictive trajectories capture higher (log-normal) noise levels by increasing the variability for larger abundances.

## (b) 5 species

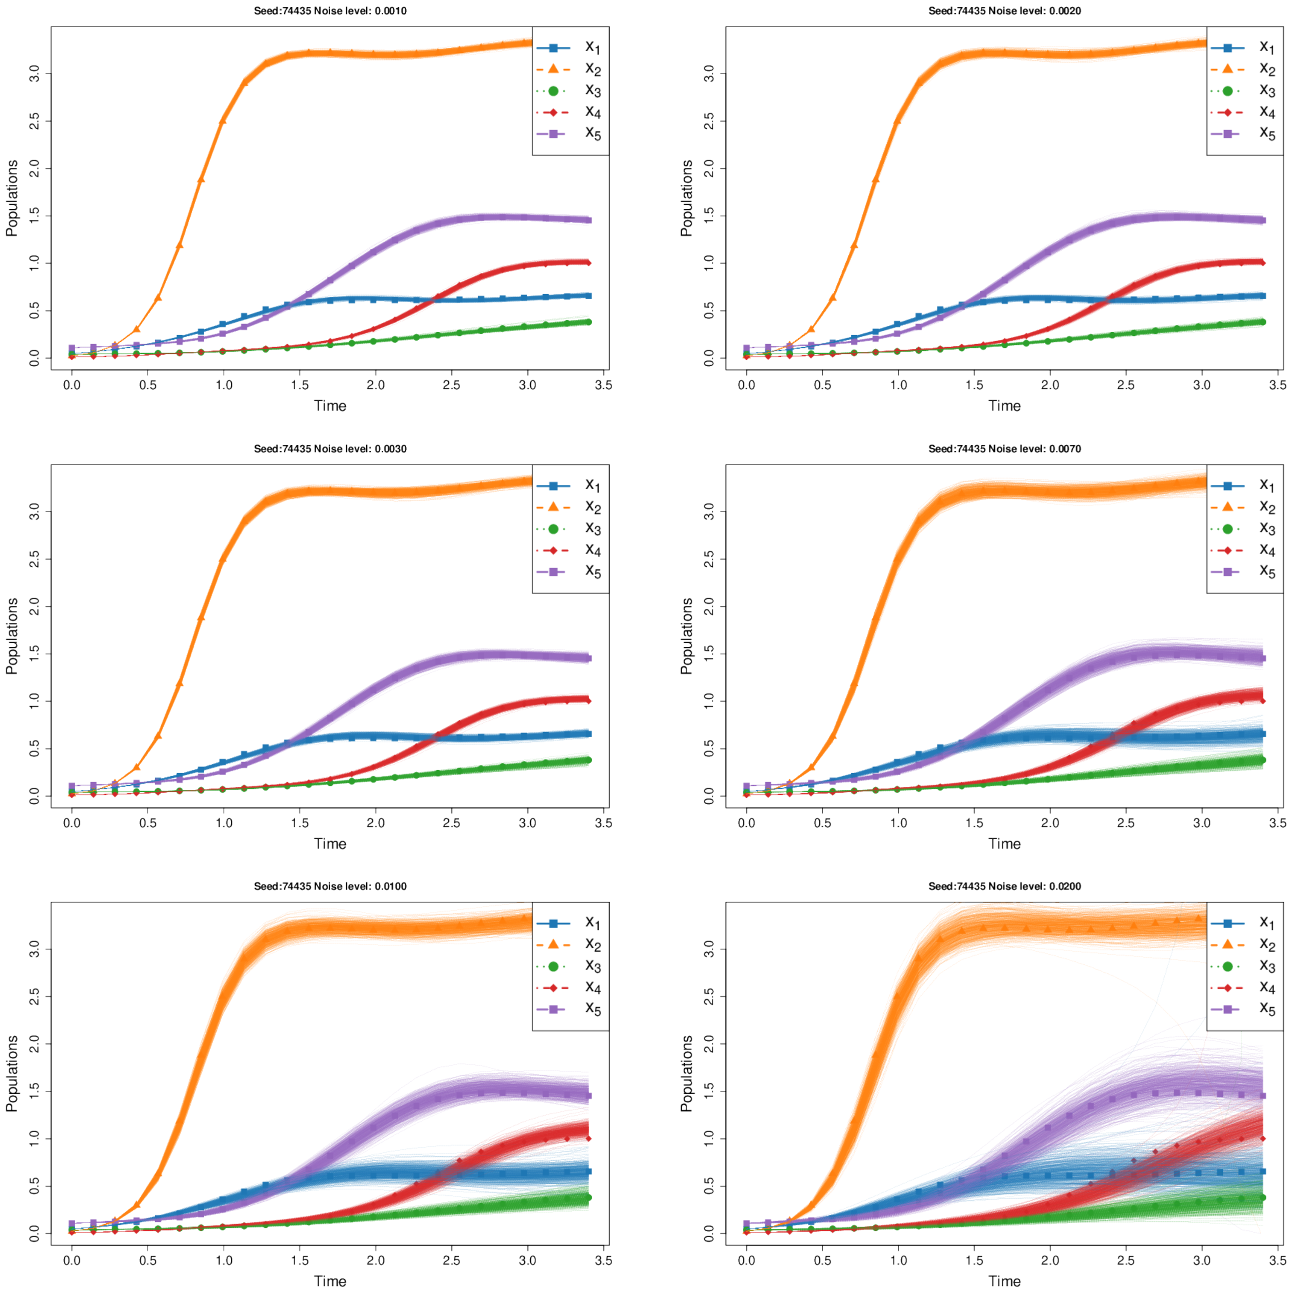


**Figure S20.** Posterior predictive trajectories simulated by sampling the posterior distributions (summarised in Sec. S3) for 6 different log-normally noise levels (title of each panel) added to the deterministic curves. The posterior predictive trajectories capture higher (log-normal) noise levels by increasing the variability for larger abundances.

## (c) 6 species

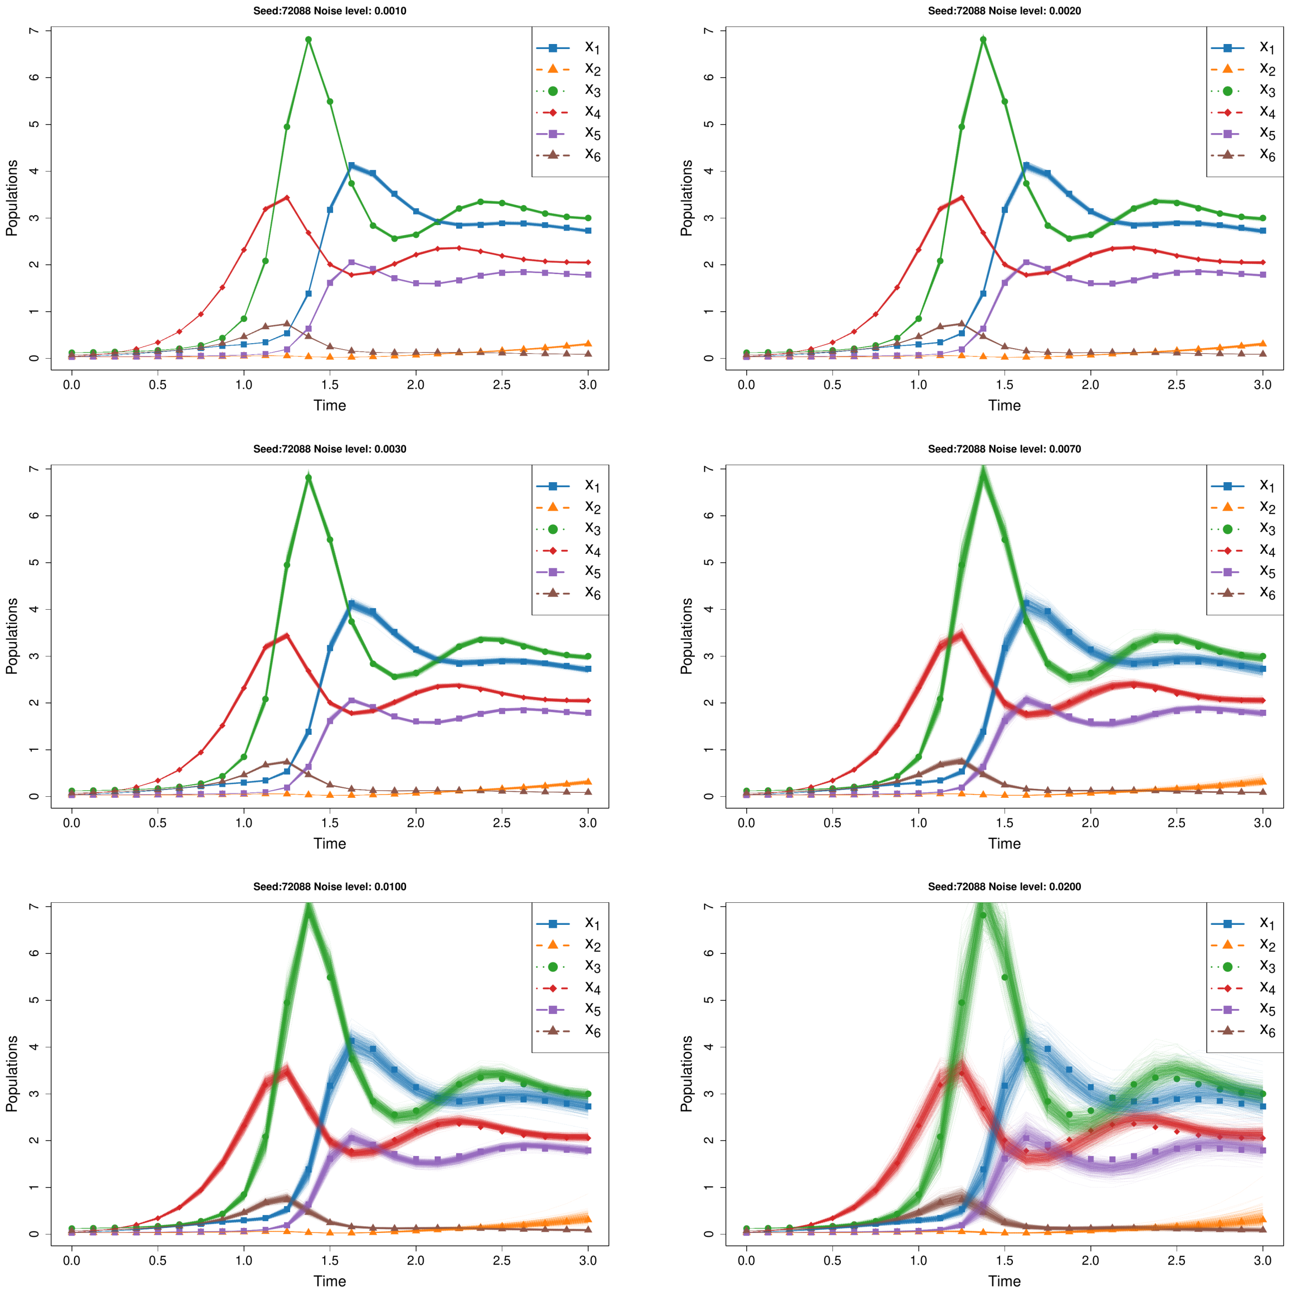


**Figure S21.** Posterior predictive trajectories simulated by sampling the posterior distributions (summarized in Sec. S3) for 6 different log-normally noise levels (title of each panel) added to the deterministic curves. The posterior predictive trajectories capture higher (log-normal) noise levels by increasing the variability for larger abundances.

# S5. Correlations between posterior marginals for 4 species

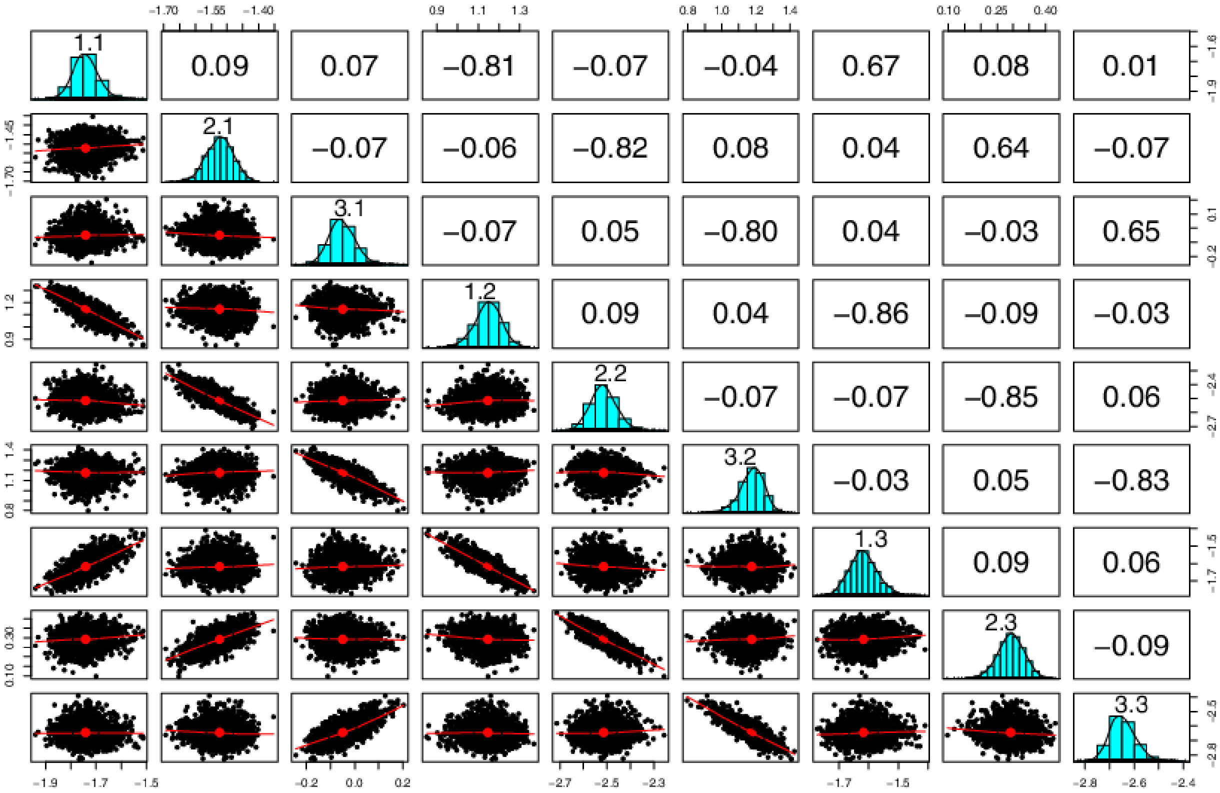

**Figure S22.** Pairs-plot of the marginal posterior distributions for the elements of the interaction matrix, $\beta_{ij}$ for 3 species, and noise level $0.007$. The label on the diagonal of the plot shows the index of the coefficient of $\beta_{ij}$. In the upper triangular part of the plot, we show the Pearson correlation between distributions. The numbers above each histogram indicate the indices of the interaction matrix. Note how the condition imposed on the parameters in order to provide positive, stable, steady-state abundances induces spurious correlations between parameters.

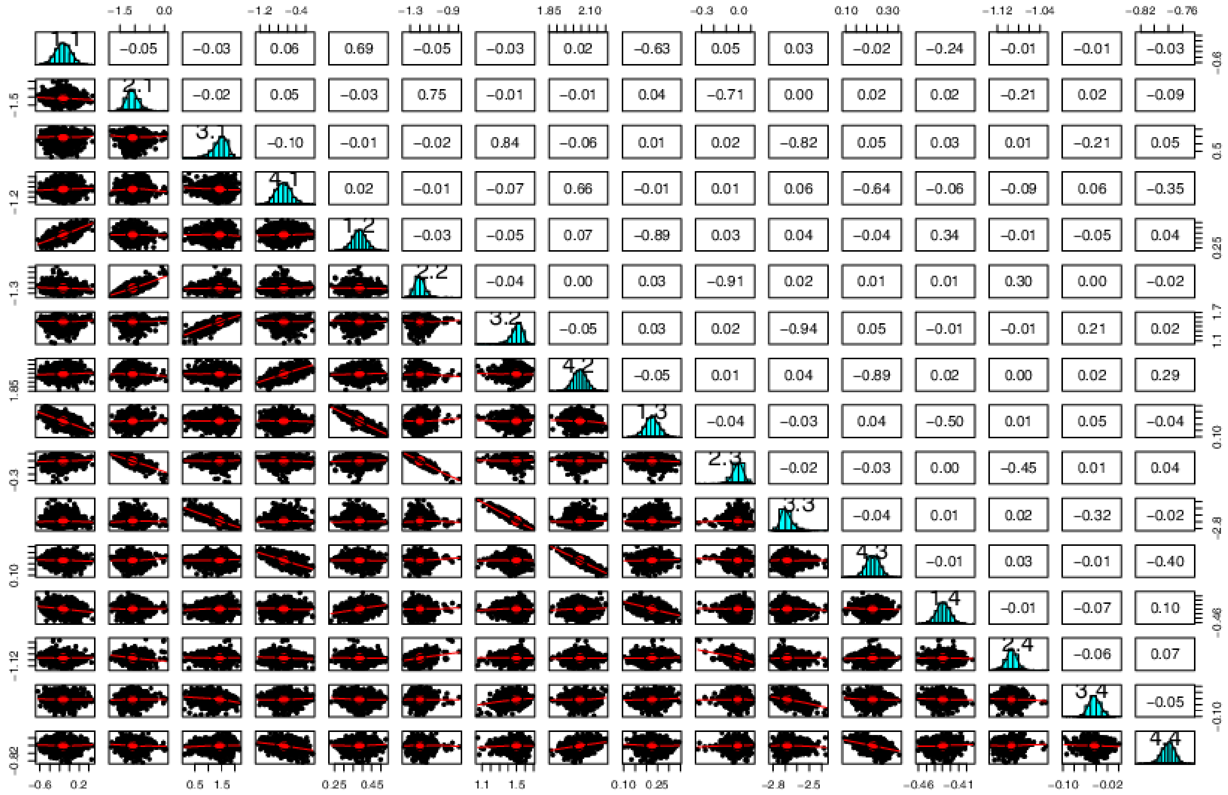

**Figure S23.** Pairs-plot of the marginal posterior distributions for the elements of the interaction matrix, $\beta_{ij}$ for 4 species, and noise level $0.003$. The label on the diagonal of the plot shows the index of the coefficient of $\beta_{ij}$. In the upper triangular part of the plot, we show the Pearson correlation between distributions. The numbers above each histogram indicate the indices of the interaction matrix. Note how the condition imposed on the parameters in order to provide positive, stable, steady-state abundances induces spurious correlations between parameters.

# S6. An example of MBAM for parameters giving periodic solutions

In Fig. S24, we show the initial and final model after applying the MBAM algorithm. The sequence provided by MBAM is as follows:

$$\beta_{33} \to 0, \beta_{22} \to 0, \beta_{23} \to 0, \text{and } \beta_{31} \to 0.$$

Further elimination provides inaccurate fitting of $x_3$ as shown in the figure.

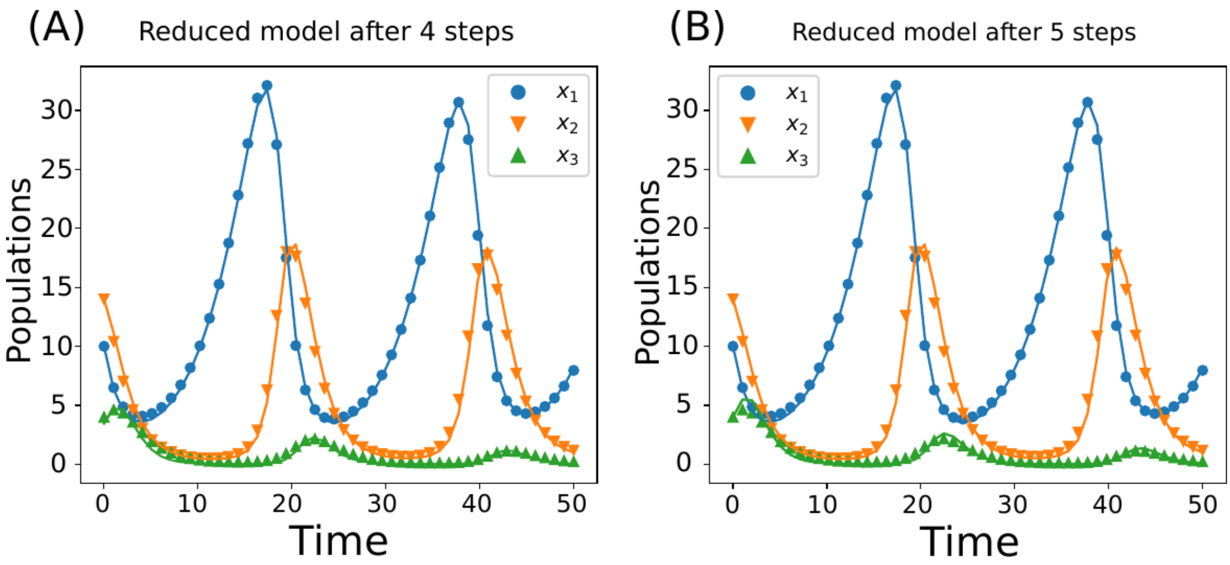


**Figure S24.** Comparison of a system entailing periodic oscillations (see parameters in Table S1) after (A) 4 MBAM and (B) 5 MBAM steps (solid lines). The symbols represent the original deterministic trajectories. Note how removing the 5th parameter fails to describe $x_3$ accurately.

# S7. Identifiability vs Sloppiness

As shown in Ref. [2], sloppiness and identifiability (practical or structural) are different concepts. The former relates to parameter meaning constrained to the information in the data, and the latter to the ability to assign a unique value to each model parameter.

In Ref. [1], the authors proved structural identifiability and illustrated that fitting relative abundances also provided practical identifiability. However, there is a caveat in their analysis: the priors used to make the Bayesian inference in that work were constrained to be between uniformly distributed 0.6 and 1.4 times the original ones, so the change in sign has probability 0.

To illustrate this, we applied MBAM to the same data parameters as in [1], which allowed us to eliminate 4 parameters while the fitting of the model is still accurate, as shown in Fig. S25. In Table S1 we collect the parameters used in the simulation. The sequence of parameters eliminated by MBAM is:

$$\beta_{33} \to 0, \beta_{21} \to 0, r_3 \to 0, \text{and } \beta_{23} \to 0,$$

but removing an additional one ($\beta_{22} \to 0$) fails to fit the model. This is insightful because it manifests that priors must be uninformative enough and that identifiability does not guarantee a lack of sloppiness and the ability to explain the data with a simpler model.

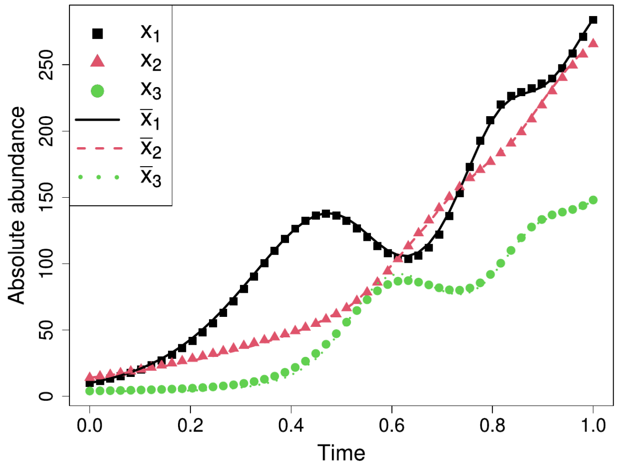


**Figure S25.** Comparison of exact simulation (symbols) of gLV model for 3 species using the same parameters as in Ref. [1] and the reduced model after 4 MBAM steps (lines). Note how, even though the model is identifiable, MBAM still purges 4 parameters while preserving the structure and idiosyncrasies of the data.

# S8. The problem of forecasting with overparametrized models

In this section, we show that fitting data for different times does not necessarily solve the problem of interpretability and sloppiness of gLV-like models. Specifically, longer time series can only help if they add more effective information than that already implicit in the shorter series. It is only through more relevant information that we can determine more parameters. But if extending the time series ends in a steady state, for instance, then it doesn't matter how many new points we add to the time series—it doesn't improve prediction.

To illustrate this, in Fig. S26, we show an example with $N = 6$ species. In Fig. S26(A), we show how the full gLV (with 42) parameters and a reduced version where we have eliminated 12 fit the data accurately for times $t <= 3$ where they have been fitted, but both predict poorly and even the full model extrapolates worse for longer times, as shown in Fig. S26(B). So, not only is the interpretability of the interactions not attainable, but more complex models also perform worse for out-of-sample data.

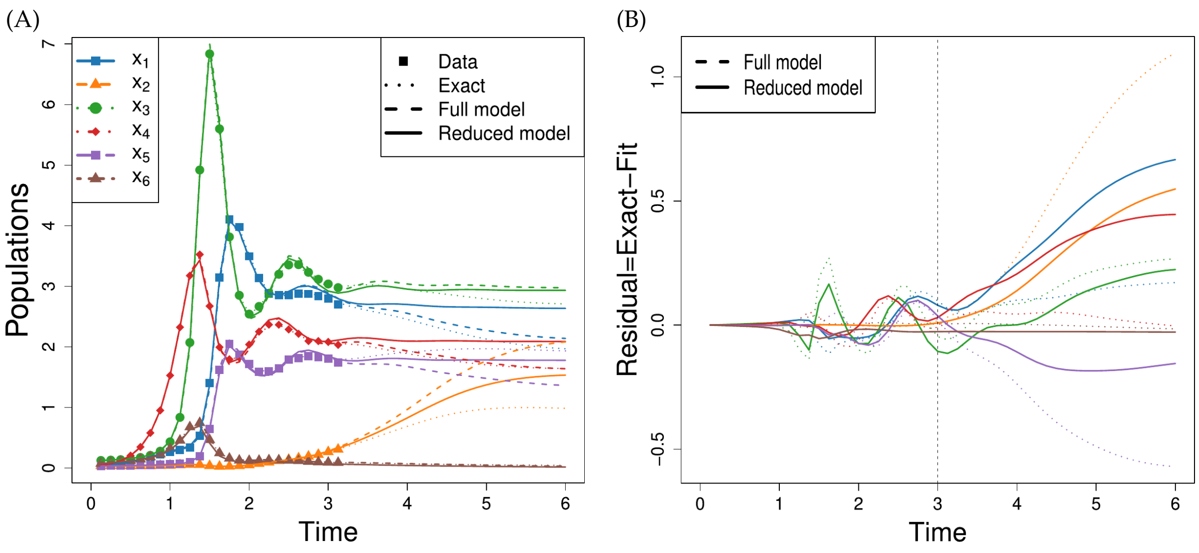


**Figure S26.** Time series obtained from a gLV model with $N = 6$ species. (A) Abundances of the species as obtained from the exact model (dotted lines), the fit to the bullet points (obtained from the exact data by adding a small amount of noise) of the full model with 42 parameters (dashed lines), and the fit to a reduced model with 30 (out of 42) non-zero parameters (full lines). (B) Difference between the abundances predicted by both fitted models (full and reduced) and the exact abundances. The vertical dotted line marks the end of the fitted data. Beyond this point, the curves are forecasting. This figure illustrates the impossibility of long-term forecasting these time series. As time passes beyond the available data, both models start forecasting poorly—the worse the longer the time.

To test this, in Fig. S27, we demonstrate why we claim that inferring parameters is doomed. The main message is that we can remove the same number of parameters, but the removed parameters in both models are different (shown in red). In particular, for shorter times, the removed parameters are

$$r_2, \beta_{12}, \beta_{22}, \beta_{25}, \beta_{32}, \beta_{42}, \beta_{52}, \beta_{54}, \beta_{61}, \beta_{62}, \beta_{65}, \beta_{66},$$

and for longer,

$$r_2, \beta_{16}, \beta_{25}, \beta_{26}, \beta_{36}, \beta_{46}, \beta_{52}, \beta_{54}, \beta_{56}, \beta_{62}, \beta_{64}, \beta_{66},$$

where those in red are missing in the other scenario. This removal procedure is computationally expensive, so for $N = 6$ we have stopped at 12 removed parameters, but extending the series does not have any effect in this case. As said above, if the longer times contain additional or richer features, we agree that there will be more relevant parameters, but this is precisely our overarching point: With poor data, you have poor estimates and ecological data is typically not rich enough (except, as suggested by Reviewer 1, the dynamics is chaotic and the whole series is contingent).

Finally, note that the time series we use are almost noiseless, so using noisier data will provide much more different estimations of the parameters, so their interpretation in microscopic terms is meaningless (as the higher experimental errors will accommodate higher variability in the set of parameters that provide curves that are close to the data).

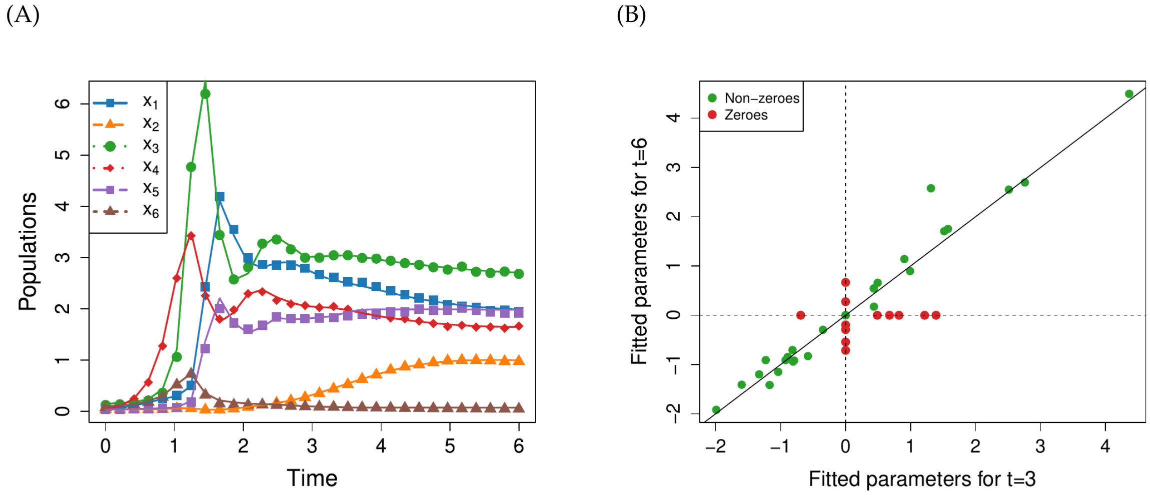


**Figure S27.** Extending the fitting time changes the interpretation of the inferred parameters. (A) Data generated (symbols) with the same (42) parameters as in Fig. S26 but extending the data until $t = 6$ and comparison with the fitting to a reduced model with just 30 parameters (solid lines). The agreement is excellent, considering the reduced model has 12 fewer parameters. (B) We compare the parameters of both reduced models (the ones fitted up to $t = 3$ and $t = 6$, respectively). The solid line is a reference line with slope 1. The dashed lines are a guide to the eye to identify those parameters that are, indeed, 0 in the reduced model obtained by fitting to times up to $t = 3$ and $t = 6$. The removed parameters in both models are different (shown in red). The fact that they lie on the lines and not on the origin shows that both sets of zero parameters are not identical.

# References

[1] C. H. Remien, M. J. Eckwright, and B. J. Ridenhour, “Structural Identifiability of the Generalized Lotka–Volterra Model for Microbiome Studies”, R. Soc. Open Sci. **8**, 201378 (2021).

[2] O.-T. Chis, A. F. Villaverde, J. R. Banga, and E. Balsa-Canto, “On the relationship between sloppiness and identifiability”, Mathematical biosciences **282**, 147–161 (2016).
